# Supplementary material for: A General Theoretical and Experimental Framework for Nanoscale Electromagnetism
Source: arXiv:1901.03988 ancillary file (2019-01-13)
Supplement: Supplementary file 1 [file supplementary.pdf]

# SUPPLEMENTARY MATERIALS

## A General Theoretical and Experimental Framework for Nanoscale Electromagnetism

Yi Yang,<sup>1,\*</sup> Di Zhu,<sup>1,\*</sup> Wei Yan,<sup>2,3</sup> Akshay Agarwal,<sup>1</sup> Mengjie Zheng,<sup>1,4</sup> John D. Joannopoulos,<sup>1</sup> Philippe Lalanne,<sup>2</sup> Thomas Christensen,<sup>1</sup> Karl K. Berggren,<sup>1</sup> and Marin Soljačić<sup>1</sup>

<sup>1</sup>Research Laboratory of Electronics, Massachusetts Institute of Technology, Cambridge, Massachusetts 02139, USA

<sup>2</sup>Laboratoire Photonique Numérique et Nanosciences, Institut d'Optique d'Aquitaine, Université Bordeaux, CNRS, 33405 Talence, France

<sup>3</sup>Institute of Advanced Technology, Westlake Institute for Advanced Study, Hangzhou 310024, China

<sup>4</sup>School of Physics and Electronics, State Key Laboratory of Advanced Design and Manufacturing for Vehicle Body, Hunan University, Changsha 410082, China

### CONTENTS

|                                                      |    |                                                                                                     |    |
|------------------------------------------------------|----|-----------------------------------------------------------------------------------------------------|----|
| Summary of framework                                 | 1  | S10. Dark field scattering measurement                                                              | 14 |
| S1. Feibelman $d$ -parameters: background            | 2  | S11. Impact of surface roughness on optical response                                                | 15 |
| S2. Derivation of mesoscopic boundary conditions     | 3  | S12. Data analysis                                                                                  | 15 |
| S3. Numerical implementation                         | 6  | S13. Index dependence of $d_{\perp}^{\text{Au-AIO}_x}$                                              | 17 |
| S4. Quasi-normal-mode perturbation theory            | 7  | S14. Additional measured Si scattering spectra                                                      | 18 |
| S5. Sample fabrication                               | 10 | S15. Al–Au results: partial cancellation of nonclassical corrections between spill-in/out materials | 18 |
| S6. Surface roughness                                | 11 | S16. TDDFT: impact of cladding screening on $d$ -parameters                                         | 20 |
| S7. Nanodisk size distribution                       | 11 | References                                                                                          | 25 |
| S8. Cross-sectional transmission electron micrograph | 12 |                                                                                                     |    |
| S9. Ellipsometry                                     | 12 |                                                                                                     |    |

### Summary of framework

In this first section, we summarize the essential elements and features of our new framework. The summary also includes a list of pointers to key related sections in the Supplementary Materials.

Application of our framework to a generic electrodynamic problem requires only three key ingredients:

1. *Identify interfaces susceptible to nonclassical corrections.* An interface  $\tau$  is composed of a boundary  $\partial\Omega^\tau$  and a pair of materials (“inside”,  $-$ , and “outside”,  $+$ ) with associated classical permittivities  $\epsilon^-$  and  $\epsilon^+$ . Interfaces which are likely to accumulate significant nonclassical corrections typically (i) host large field gradients (i.e. rapidly varying or extremely confined fields), (ii) feature small geometric scales (possibly nearby), and (iii) comprise at least one metallic material.
2. *Pair each interface with associated Feibelman  $d$ -parameters.* The Feibelman  $d_{\perp}$ - and  $d_{\parallel}$ -parameters are functions of the interface’s material-composition and the frequency  $\omega$  (for background, see Sec. S1). The specific functional dependence of the  $d$ -parameters can be obtained by:

*First-principles calculations.* Time-dependent density functional theory (TDDFT) and linear response-theory enable the computational evaluation of  $d$ -parameters (see Sec. S16). Simple metals are well-described by an unscreened jellium approximation. In noble metals, valence-electron screening is non-negligible, requiring incorporation of lower-lying orbitals or use of semiclassically screened jellium approaches.

*Measurements.* As an alternative to computation,  $d$ -parameters can be measured in suitably designed setups, in a manner analogous to that of ellipsometry. Our experiment, detailed in the main text and in Secs. S5–S13, showcase the utility and versatility of this approach.

3. *Incorporate  $d$ -parameters into electromagnetic response.* The Feibelman  $d$ -parameters modify the

classical boundary conditions (BCs), which, as discussed in the main text, are supplanted by a set of mesoscopic BCs (see Sec. S2). At coordinates away from the interface, i.e. at  $\mathbf{r} \notin \partial\Omega^\tau$ , the usual macroscopic Maxwell equations apply. We have developed and used two complementary techniques to incorporate the impact of these new BCs:

*Direct incorporation in numerical solver.* The new BCs can be directly incorporated in existing electromagnetic numerical solvers. Concretely, we have implemented the new BCs in the popular solver COMSOL Multiphysics (see Sec. S3), enabling calculation of virtually every electromagnetic (linear-)response quantity.

*Quasi-normal-mode-based perturbation theory.* We have developed a perturbation theoretical expression for the nonclassical spectral shift,  $\tilde{\omega}^{(1)}$ , expanded on quasi-normal modes (QNMs; see Sec. S4). The shift's magnitude is determined by interface-summed product of  $d$ -parameters and a set of nonclassical perturbation amplitudes  $\kappa_{\perp,\parallel}^\tau$ . The latter can be calculated from the classical eigenproblem's QNMs, using only the fields at the interface's boundary.

A set of representative COMSOL Multiphysics examples will be made freely available upon publication, allowing direct transfer of the methodology to a broad variety of setups.

## S1. FEIBELMAN $d$ -PARAMETERS: BACKGROUND

The Feibelman  $d$ -parameters have been extensively treated in past literature [S1–S3], and also recently studied by some of the authors of this paper [S4]. Here, we provide a brief summary of their definitions, properties, and implications.

One appealing approach to introduce the  $d$ -parameters—and the one taken by Feibelman—is by analysis of the reflection of an external potential off a planar interface: the  $d$ -parameters then emerge as parametrizations of the leading-order correction to the classical reflection coefficient. Concretely, we consider a planar interface at  $x = 0$ , extended along  $\mathbf{r}_\parallel = (y, z)$ , separating semi-infinite, homogeneous materials on either side.\* An external potential  $\phi^{\text{ext}}(\mathbf{r}) = e^{iky+kx}$  (with an implicit  $e^{-i\omega t}$  frequency dependence) is assumed incident onto the interface from  $x > 0$ . In response, an induced potential  $\phi^{\text{ind}}(\mathbf{r}) = e^{iky}\phi^{\text{ind}}(x)$  is instated: on the  $x > 0$  side, this induced potential is simply a reflected part. While classically, the reflected potential is just  $\phi^{\text{ind}}(x > 0) = r^c e^{-kx}$ —with  $r^c$  denoting the classical reflection coefficient—the quantum-mechanical reality is less simple. Rather, near the interface  $\phi^{\text{ind}}(x)$  is generally complicated: this is because the overall response is not rigorously characterized by a sudden step-change in local bulk permittivities  $\varepsilon^-$  and  $\varepsilon^+$  (applicable to the regions  $x < 0$  and  $x > 0$ , respectively), as is assumed classically, but instead characterized by a smoothly varying, nonlocal permittivity  $\varepsilon(\mathbf{r}, \mathbf{r}') = \varepsilon(\mathbf{r}_\parallel - \mathbf{r}'_\parallel; x, x')$ . Far away from  $x = 0$  (with “far away” defined, of course, relative to the intrinsic electronic length scales characterizing the interface), however, the  $x$ -dependence of the reflected potential must again follow the classical prediction, since, locally, translation invariance is gradually restored for  $x \gg 0$ . In other words, the asymptotic dependence of the actual reflected potential parallels the classical one, i.e.  $\phi^{\text{ind}}(x \gg 0) \simeq r e^{-kx}$ —but, crucially, with a different reflection amplitude,  $r \neq r^c$ . The Feibelman  $d$ -parameters emerge naturally in the derivation of this reflection coefficient if one consistently retains only the leading-order (i.e.  $O(k)$ ) corrections to the classical response. Specifically, one finds that (see e.g. Ref. S4):

$$r = -\frac{(\varepsilon^- - \varepsilon^+) + (\varepsilon^- - \varepsilon^+)(d_\perp + d_\parallel)k}{(\varepsilon^- + \varepsilon^+) - (\varepsilon^- - \varepsilon^+)(d_\perp - d_\parallel)k} + O(k^2), \quad (\text{S1a})$$

where

$$d_\perp = \frac{\int_{-\infty}^{\infty} x \rho(x) dx}{\int_{-\infty}^{\infty} \rho(x) dx}, \quad d_\parallel = \frac{\int_{-\infty}^{\infty} x \partial_y J_y(x) dx}{\int_{-\infty}^{\infty} \partial_y J_y(x) dx}. \quad (\text{S1b})$$

with  $e^{iky}\rho(x)$  and  $e^{iky}\mathbf{J}(x) = e^{iky}(J_x, J_y, J_z)(x)$  denoting the *quantum-mechanical* induced charge and current due to the external potential  $\phi^{\text{ext}}(\mathbf{r}) = e^{iky+kx}$ .

---

\* Though not formally necessary, it is convenient to consider the side  $x < 0$  as the metallic side here: this establishes a connection between the signs of the  $d$ -parameters and the conceptual notions of charge spill-in and spill-out

Several facts bear mentioning:

1.  $d_{\perp}$  and  $d_{\parallel}$  correspond, respectively, to the centroid of induced charge density and centroid of the in-plane derivative of the in-plane current density. They have units of length.
2. Since the induced response,  $\rho(x)$  and  $J_y(x)$ , depends on the external potential's frequency and the interface's composition, as do the  $d$ -parameters. In the frequency-domain, the  $d$ -parameters are consequently complex quantities (and subject to Kramers–Kronig relations [S5]).
3. Since the induced response also depends on the wave vector  $k$  of the external perturbation  $\phi^{\text{ext}}$ , Eq. (S1b) must be augmented with a choice of  $k$ . The appropriate choice,  $k \rightarrow 0$ , follows naturally from the leading-order  $O(k)$  scope of the procedure: inclusion of  $k$ -dependence in the  $d$ -parameters beyond the  $O(1)$ -term contributes only to  $O(k^2)$  terms, i.e. is negligible.
4. The  $d$ -parameters are not properties of a single material: rather, they are (intensive) properties of the two materials that make up the interface.<sup>†</sup>
5.  $d_{\perp}$  is of much greater practical relevance than  $d_{\parallel}$ . Specifically, it has been shown that  $d_{\parallel}$  vanishes at charge-neutral jellium interfaces [S3]; similarly, it can be shown that  $d_{\parallel}$  vanishes for charge-neutral interfaces with periodic ionic potentials. Thus, it is reasonably expected that  $|d_{\perp}| \gg |d_{\parallel}|$  even for non-idealized, charge-neutral interfaces. Still, it is useful to retain  $d_{\parallel}$  in the analysis as it can enable effective treatments of bound screening [S6; S7], surface roughness [S8], and surface-adsorbates.

The qualitative impact of the  $d$ -parameters can be appreciated readily by considering the modifications to the surface plasmon resonance frequency of a simple jellium–vacuum interface (where  $\varepsilon^- = 1 - \omega_p^2/\omega^2$  and  $\varepsilon^+ = 1$ ). The resonance condition follows from the poles of Eq. (S1a), allowing

$$\begin{aligned}\omega_{\text{sp}} &= \omega_{\text{sp}}^c \sqrt{1 - kd_{\perp}(\omega_{\text{sp}}) + kd_{\parallel}(\omega_{\text{sp}})} \\ &\simeq \omega_{\text{sp}}^c \left[ 1 - \frac{1}{2}kd_{\perp}(\omega_{\text{sp}}^c) + \frac{1}{2}kd_{\parallel}(\omega_{\text{sp}}^c) \right],\end{aligned}\quad (\text{S2})$$

where  $\omega_{\text{sp}}^c = \omega_p/\sqrt{2}$  is the classical surface plasmon frequency, and where, at the approximate equality, the assumed smallness of  $kd_{\perp,\parallel}$  justifies a first-order Taylor expansion and a pole-approximation. Focusing on  $d_{\perp}$ , Eq. (S2) shows that if  $\text{Re } d_{\perp} < 0$  (the induced charge's centroid is inside the metal, i.e. spill-in) the resonance blueshifts; conversely, if  $\text{Re } d_{\perp} > 0$  (spill-out) the resonance redshifts. Moreover,  $\text{Im } d_{\perp}$  (a positive quantity below the plasma frequency) evidently contributes broadening. This broadening is physically due to surface-enabled Landau damping—i.e. nonvertical, intraband electron-hole pair excitations, with the necessary momentum supplied by the termination of translation invariance at the interface.

## S2. DERIVATION OF MESOSCOPIC BOUNDARY CONDITIONS

### A. Feibelman $d$ -parameters as surface polarizations

Ref. S4 established that—within a nonretarded scope—the  $d_{\perp}$ - and  $d_{\parallel}$ -parameters can be incorporated as an induced (out-of-plane) surface polarization  $\boldsymbol{\pi}$  and an induced (in-plane) surface current  $\mathbf{K}$ . Specifically, the induced surface quantities equal (implicitly evaluated at an interface coordinate  $\mathbf{r}_{\parallel}$ )

$$\boldsymbol{\pi} = -\varepsilon_0 d_{\perp} \llbracket \nabla_{\perp} \phi \rrbracket \hat{\mathbf{n}}, \quad (\text{S3a})$$

$$\mathbf{K} = -i\varepsilon_0 \omega d_{\parallel} \llbracket \varepsilon \nabla_{\parallel} \phi \rrbracket, \quad (\text{S3b})$$

with total, self-consistent potential  $\phi(\mathbf{r})$  (including impact of Feibelman  $d$ -parameters), “outside–inside” interface discontinuities  $\llbracket \nabla_{\perp} \phi \rrbracket \equiv \nabla_{\perp} \phi(\mathbf{r}_{\parallel}^+) - \nabla_{\perp} \phi(\mathbf{r}_{\parallel}^-)$  and  $\llbracket \varepsilon \nabla_{\parallel} \phi \rrbracket \equiv \varepsilon^+ \nabla_{\parallel} \phi(\mathbf{r}_{\parallel}^+) - \varepsilon^- \nabla_{\parallel} \phi(\mathbf{r}_{\parallel}^-)$  [with local,

---

<sup>†</sup> In principle, the  $d$ -parameters also depend on the relative orientation of the two materials as well as possible atomic reconstructions in the surface region (i.e. surface reconstruction).

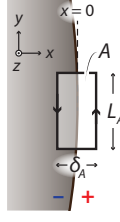

**Figure S1. Integration box in Eq. (‡1):** the length  $\delta_A$  is assumed vanishingly small, and the length  $L_A$  is assumed small compared to any variations of any field- or source-terms as well as the geometric curvature.

bulk permittivities  $\varepsilon^+$  “outside” (i.e. at  $\mathbf{r}_{\parallel}^+ \equiv \mathbf{r}_{\parallel} + 0^+ \hat{\mathbf{n}}$ ) and  $\varepsilon^-$  “inside” (i.e. at  $\mathbf{r}_{\parallel}^- \equiv \mathbf{r}_{\parallel} - 0^+ \hat{\mathbf{n}}$ ) the interface], and outward normal vector  $\hat{\mathbf{n}}$ .

The retarded generalization of Eqs. (S3) is nearly immediate: Eq. (S3a) generalizes trivially, since  $-\nabla\phi \rightarrow \mathbf{E}$  in the retarded formulation. Thus,

$$\boldsymbol{\pi} = \varepsilon_0 d_{\perp} \llbracket E_{\perp} \rrbracket \hat{\mathbf{n}}. \quad (\text{S4a})$$

A similar generalization of Eq. (S3b) might initially seem impermissible: though  $-\varepsilon_0 \varepsilon \nabla\phi \rightarrow \mathbf{D}$  classically, this is no longer rigorously the case when including  $d$ -parameters (because  $\varepsilon$  refers to local, bulk permittivities). Once again, recalling the strict first-order scope of the approach is helpful: the difference between the classical and Feibelman-corrected  $\mathbf{D}$ -field is first order—as is  $\mathbf{K}$  itself, cf. its linear proportionality to  $d_{\parallel}$ . The difference between  $\mathbf{K}$  sourced by classical and Feibelman-corrected  $\mathbf{D}$ -fields is thus *second* order, i.e. negligible in our first-order scope. The naïve replacement is then permissible, allowing

$$\mathbf{K} = i\omega d_{\parallel} \llbracket \mathbf{D}_{\parallel} \rrbracket. \quad (\text{S4b})$$

It is interesting to note that the nonclassical source terms  $\boldsymbol{\pi}$  and  $\mathbf{K}$  are sourced by the field-discontinuities across the interface. Notably, in a fully quantum-mechanical treatment, the fields are continuous everywhere; the discontinuities in the classical approach are consequences of the local-response approximation  $\varepsilon(\mathbf{r}, \mathbf{r}') \simeq \delta(\mathbf{r} - \mathbf{r}')\varepsilon(\mathbf{r})$  with  $\varepsilon(\mathbf{r})$  discontinuous at interfaces. It is arguably both natural and appealing to find the leading-order corrections of this approximation intimately tied to its consequences.

## B. Feibelman $d$ -parameters as boundary conditions

*Summary* First, we restate the mesoscopic boundary conditions (BCs; Fig. 1b) for ease of reference:

$$\llbracket \mathbf{H}_{\parallel} \rrbracket = \mathbf{K} \times \hat{\mathbf{n}} = i\omega d_{\parallel} \llbracket \mathbf{D}_{\parallel} \rrbracket \times \hat{\mathbf{n}}, \quad (\text{S5a})$$

$$\llbracket D_{\perp} \rrbracket = (i\omega)^{-1} \nabla_{\parallel} \cdot \mathbf{K} = d_{\parallel} \nabla_{\parallel} \cdot \llbracket \mathbf{D}_{\parallel} \rrbracket, \quad (\text{S5b})$$

$$\llbracket \mathbf{E}_{\parallel} \rrbracket = -\varepsilon_0^{-1} \nabla_{\parallel} \boldsymbol{\pi} = -d_{\perp} \nabla_{\parallel} \llbracket E_{\perp} \rrbracket, \quad (\text{S5c})$$

$$\llbracket B_{\perp} \rrbracket = 0. \quad (\text{S5d})$$

*Surface current density* Incorporating an in-plane surface current density  $\mathbf{K}$  in the macroscopic Maxwell boundary conditions (BCs) is a text-book matter<sup>‡</sup> [S9]— $\llbracket \mathbf{H}_{\parallel} \rrbracket = \mathbf{K} \times \hat{\mathbf{n}}$  and  $\llbracket D_{\perp} \rrbracket = (i\omega)^{-1} \nabla_{\parallel} \cdot \mathbf{K}$ —allowing immediate transposition of Eq. (S4b) to Eqs. (S5a) and (S5b).

<sup>‡</sup> By Stokes’ theorem and the Maxwell–Ampere equation,  $\nabla \times \mathbf{H} = \mathbf{J} + \partial_t \mathbf{D}$ , one has (with the integration box  $A$  in Fig. S1)

$$\int_A \nabla \times \mathbf{H}(\mathbf{r}) \cdot d\mathbf{A} = \int_{\partial A} \mathbf{H}(\mathbf{r}) \cdot d\mathbf{l} = \int_A \mathbf{K}(\mathbf{r}_{\parallel}) \delta(z) \cdot d\mathbf{A} - \int_A i\omega \mathbf{D}(\mathbf{r}) \cdot d\mathbf{A}. \quad (\text{‡1})$$

Taking  $(L_A, \delta_A) \rightarrow 0$  while keeping  $L_A \gg \delta_A$  this simplifies to  $H_y(\mathbf{r}_{\parallel}^+) - H_y(\mathbf{r}_{\parallel}^-) = K_z(\mathbf{r}_{\parallel})$ . Similarly, by rotating the integration box  $A$ , one finds  $-H_z(\mathbf{r}_{\parallel}^+) + H_z(\mathbf{r}_{\parallel}^-) = K_y(\mathbf{r}_{\parallel})$ . Evidently, this generalizes to  $\llbracket \mathbf{H}_{\parallel} \rrbracket = \mathbf{K} \times \hat{\mathbf{n}}$ .

Analogously, by the divergence theorem, the continuity equation,  $\nabla_{\parallel} \cdot \mathbf{K} = i\omega\sigma$ , and the electric Gauss law,  $\nabla \cdot \mathbf{D} = \rho = \delta(z)\sigma$  (with surface charge density  $\sigma$ ) one finds (by integrating over an infinitesimal interface-enclosing volume)  $\llbracket D_{\perp} \rrbracket = \sigma = (i\omega)^{-1} \nabla_{\parallel} \cdot \mathbf{K}$ .

*Surface dipole density* Incorporating an out-of-plane surface dipole density  $\pi$  is, by comparison, less commonplace—albeit occasionally featured in introductions to electrostatics [S10]. In a retarded setting, it can be derived by considering the fields radiated by the self-consistent bulk and surface currents (see also Ref. S11):

$$\begin{aligned} \mathbf{E}(\mathbf{r}) &= i\omega\mu_0 \int \mathbf{G}_0(\mathbf{r}, \mathbf{r}') \mathbf{J}_{\text{tot}}(\mathbf{r}') d^3\mathbf{r}' \\ &= \underbrace{i\omega\mu_0 \int_{\mathbb{R}^3} \mathbf{G}_0(\mathbf{r}, \mathbf{r}') \mathbf{J}_{\text{bulk}}(\mathbf{r}') d^3\mathbf{r}'}_{\text{bulk polarization current}} + \underbrace{i\omega\mu_0 \int_{\partial\Omega} \mathbf{G}_0(\mathbf{r}, \mathbf{r}') \mathbf{K}(\mathbf{r}') d^2\mathbf{r}'}_{\text{surface current density}} + \underbrace{\omega^2\mu_0 \int_{\partial\Omega} \mathbf{G}_0(\mathbf{r}, \mathbf{r}') \pi(\mathbf{r}') d^2\mathbf{r}'}_{\text{surface dipole density}}, \end{aligned} \quad (\text{S6})$$

with dyadic free-space Green function  $\mathbf{G}_0(\mathbf{r}, \mathbf{r}') = (\mathbf{1} + k_0^{-2} \nabla \nabla^T) g_0(\mathbf{r}, \mathbf{r}')$ , defined in terms of the scalar free-space Green function  $g_0(\mathbf{r}, \mathbf{r}') = e^{ik_0|\mathbf{r}-\mathbf{r}'|}/4\pi|\mathbf{r}-\mathbf{r}'|$ , free-space wave vector  $k_0 = \omega/c$ , and with induced bulk currents  $\mathbf{J}_{\text{bulk}}(\mathbf{r}) = -i\omega\epsilon_0[\epsilon(\mathbf{r}) - 1]\mathbf{E}(\mathbf{r})$ . We seek a replacement for the classical BC  $\llbracket \mathbf{E}_{\parallel} \rrbracket = 0$ . This replacement can be found via Eq. (S6) by evaluating  $\lim_{\delta \rightarrow 0^+} \mathbf{E}_{\parallel}(\mathbf{r}_{\parallel} + \delta \hat{\mathbf{n}}) - \mathbf{E}_{\parallel}(\mathbf{r}_{\parallel} - \delta \hat{\mathbf{n}})$ . A significant simplification can be made immediately since we know (from the classical analysis) that neither bulk polarizations nor in-plane surface currents lead to a discontinuity in  $\mathbf{E}_{\parallel}$ : consequently, we can drop those terms straightaway—any discontinuity in  $\mathbf{E}_{\parallel}$  must be solely due to  $\pi$

$$\begin{aligned} \llbracket \mathbf{E}_{\parallel} \rrbracket &= \lim_{\delta \rightarrow 0^+} [\mathbf{E}(\mathbf{r}_{\parallel} + \delta \hat{\mathbf{n}}) - \mathbf{E}(\mathbf{r}_{\parallel} - \delta \hat{\mathbf{n}})]_{\parallel} \\ &= \omega^2\mu_0 \lim_{\delta \rightarrow 0^+} \left\{ \int_{\partial\Omega} [\mathbf{G}_0(\mathbf{r}_{\parallel} + \delta \hat{\mathbf{n}}, \mathbf{r}') - \mathbf{G}_0(\mathbf{r}_{\parallel} - \delta \hat{\mathbf{n}}, \mathbf{r}')] \pi(\mathbf{r}') d^2\mathbf{r}' \right\}_{\parallel}. \end{aligned} \quad (\text{S7})$$

Next, we exploit the properties of the dyadic free-space Green function, which, after several manipulations,<sup>§</sup> allows re-expressing the field due to the surface dipole density at points  $\mathbf{r} \notin \partial\Omega$

$$\mathbf{E}[\pi](\mathbf{r}) = \omega^2\mu_0 \int_{\partial\Omega} \mathbf{G}_0(\mathbf{r}, \mathbf{r}') \pi(\mathbf{r}') d^2\mathbf{r}' = \epsilon_0^{-1} \int_{\partial\Omega} [\nabla g_0(\mathbf{r}, \mathbf{r}')] \times [\nabla' \times \pi(\mathbf{r}')] d^2\mathbf{r}'. \quad (\text{S8})$$

By combining Eq. (S8) and (S7), we obtain

$$\llbracket \mathbf{E}_{\parallel} \rrbracket = \epsilon_0^{-1} \lim_{\delta \rightarrow 0^+} \left\{ \int_{\partial\Omega} [\nabla g_0(\mathbf{r}_{\parallel} + \delta \hat{\mathbf{n}}, \mathbf{r}') - \nabla g_0(\mathbf{r}_{\parallel} - \delta \hat{\mathbf{n}}, \mathbf{r}')] \times [\nabla' \times \pi(\mathbf{r}')] d^2\mathbf{r}' \right\}_{\parallel}. \quad (\text{S9})$$

<sup>§</sup> The reductions require several steps [below, an  $(\mathbf{r}, \mathbf{r}')$ -dependence is implicit in every Green function, i.e. in  $\mathbf{G}_0$  and  $g_0$ , and  $\mathbf{r}'$ -dependence is implicit in every generic current term  $\mathbf{J}$ , and an  $\mathbf{r}'_{\parallel}$ -dependence is implicit in every dipole density term  $\pi$ ]:

1. Since  $\mathbf{r} \neq \mathbf{r}'$  everywhere (cf.  $\mathbf{r} \notin \partial\Omega$ ) and since  $\nabla \times \nabla \times \mathbf{G}_0 - k_0^2 \mathbf{G}_0 = \mathbf{1}\delta(\mathbf{r} - \mathbf{r}')$ , we have  $\mathbf{G}_0 = k_0^{-2} \nabla \times \nabla \times \mathbf{G}_0$ .
2. The connection between  $\mathbf{G}_0$  and  $g_0$  allows  $\mathbf{G}_0 = k_0^{-2} \nabla \times \nabla \times [(\mathbf{1} + k_0^{-2} \nabla \nabla^T) g_0] = k_0^{-2} \nabla \times \nabla \times (g_0 \mathbf{1})$ .
3. Given the  $\mathbf{r} \leftrightarrow -\mathbf{r}'$  symmetry of  $g_0$ , we may swap  $\nabla \times$  for  $-\nabla' \times$ , such that  $\mathbf{G}_0 = -k_0^{-2} \nabla \times \nabla' \times (g_0 \mathbf{1})$ .
4. The field due to some current density  $\mathbf{J}$  is then

$$\begin{aligned} \mathbf{E}[\mathbf{J}](\mathbf{r}) &= (i\epsilon_0\omega)^{-1} \nabla \times \int_{\mathbb{R}^3} [\nabla' \times (g_0 \mathbf{1})] \mathbf{J} d^3\mathbf{r}' && \text{moving } \nabla \times \text{ outside the integral} \\ &= (i\epsilon_0\omega)^{-1} \nabla \times \int_{\mathbb{R}^3} (\nabla' g_0) \times \mathbf{J} d^3\mathbf{r}'. && \text{cf. } \nabla \times (f \mathbf{1}) = (\nabla f) \times \mathbf{1} \text{ (dyadic identity)} \\ &= (i\epsilon_0\omega)^{-1} \nabla \times \int_{\mathbb{R}^3} \nabla' \times (g_0 \mathbf{J}) - g_0 (\nabla' \times \mathbf{J}) d^3\mathbf{r}' && \text{cf. } \nabla \times (f \mathbf{A}) = (\nabla f) \times \mathbf{A} + f (\nabla \times \mathbf{A}) \\ &= -(i\epsilon_0\omega)^{-1} \nabla \times \int_{\mathbb{R}^3} g_0 (\nabla' \times \mathbf{J}) d^3\mathbf{r}' && \text{cf. } \int_{\Omega} \nabla \times \mathbf{A} d^3\mathbf{r} = \int_{\partial\Omega} \hat{\mathbf{n}} \times \mathbf{A} d^2\mathbf{r} = 0 \text{ since } \Omega = \mathbb{R}^3 \Rightarrow \partial\Omega = \emptyset \\ &= -(i\epsilon_0\omega)^{-1} \int_{\mathbb{R}^3} (\nabla g_0) \times (\nabla' \times \mathbf{J}) d^3\mathbf{r}'. \end{aligned} \quad (\text{§1})$$

5. Finally, we substitute  $\mathbf{J} = -i\omega\pi\delta(\mathbf{r}' - \partial\Omega)$  (i.e.  $\propto$  a surface Dirac function) and manipulate the resulting term  $\nabla' \times \mathbf{J} = -i\omega\nabla' \times [\pi\delta(\mathbf{r}' - \partial\Omega)]$ . To do so, we split  $\nabla = \nabla_{\parallel} + \nabla_{\perp}$  into tangential  $\nabla_{\parallel} = (\mathbf{1} - \hat{\mathbf{n}}\hat{\mathbf{n}}^T)\nabla$  and normal  $\nabla_{\perp} = \hat{\mathbf{n}}\hat{\mathbf{n}}^T\nabla$  components. For an analogously defined vector  $\mathbf{A} = \mathbf{A}_{\parallel} + \mathbf{A}_{\perp}$  the curl is then  $\nabla \times \mathbf{A} = (\nabla_{\parallel} + \nabla_{\perp}) \times (\mathbf{A}_{\parallel} + \mathbf{A}_{\perp}) = \nabla_{\parallel} \times \mathbf{A}_{\perp} + \nabla_{\perp} \times \mathbf{A}_{\parallel}$  since mutually parallel terms vanish. Then, since  $\pi \propto \hat{\mathbf{n}}$  (i.e.  $\pi_{\parallel} = 0$ ) we have  $\nabla' \times \mathbf{J} = -i\omega\nabla'_{\parallel} \times [\pi\delta(\mathbf{r}' - \partial\Omega)]$  and since  $\delta(\mathbf{r}' - \partial\Omega)$  only varies in the  $\hat{\mathbf{n}}$  direction, it can be moved outside:  $\nabla' \times \mathbf{J} = -i\omega\delta(\mathbf{r}' - \partial\Omega)\nabla'_{\parallel} \times \pi$ . Lastly, since  $\pi$  only varies along tangential directions, we can substitute  $\nabla'_{\parallel} \times$  for  $\nabla' \times$ . Using this in Eq. (§1) then yields Eq. (S8).

Since  $\nabla g_0(\mathbf{r}, \mathbf{r}')$  is a smooth function, the integrand is vanishingly small for  $\delta \rightarrow 0^+$ , except in an infinitesimal region near  $\mathbf{r}'_{\parallel} \rightarrow \mathbf{r}_{\parallel}$  where  $\nabla g_0(\mathbf{r}, \mathbf{r}')$  is singular. Exploiting this, Eq. (S9) simplifies to

$$\begin{aligned} \llbracket \mathbf{E}_{\parallel} \rrbracket &= \varepsilon_0^{-1} \lim_{\delta \rightarrow 0^+} \left\{ \int_{\partial\Omega} [\nabla g_0(\mathbf{r}_{\parallel} + \delta \hat{\mathbf{n}}, \mathbf{r}'_{\parallel}) - \nabla g_0(\mathbf{r}_{\parallel} - \delta \hat{\mathbf{n}}, \mathbf{r}'_{\parallel})] d^2 \mathbf{r}'_{\parallel} \times [\nabla \times \boldsymbol{\pi}(\mathbf{r}_{\parallel})] \right\}_{\parallel} \\ &= -\frac{1}{4\pi\varepsilon_0} \lim_{\delta \rightarrow 0^+} \left\{ \int_{\partial\Omega} \left[ \frac{\mathbf{r}_{\parallel} + \delta \hat{\mathbf{n}} - \mathbf{r}'_{\parallel}}{|\mathbf{r}_{\parallel} + \delta \hat{\mathbf{n}} - \mathbf{r}'_{\parallel}|^3} - \frac{\mathbf{r}_{\parallel} - \delta \hat{\mathbf{n}} - \mathbf{r}'_{\parallel}}{|\mathbf{r}_{\parallel} - \delta \hat{\mathbf{n}} - \mathbf{r}'_{\parallel}|^3} \right] d^2 \mathbf{r}'_{\parallel} \times [\nabla \times \boldsymbol{\pi}(\mathbf{r}_{\parallel})] \right\}_{\parallel} \\ &= -\frac{1}{4\pi\varepsilon_0} \lim_{\delta \rightarrow 0^+} \left\{ \int_{\partial\Omega} \frac{2\delta \hat{\mathbf{n}}}{[|\mathbf{r}_{\parallel} - \mathbf{r}'_{\parallel}|^2 + \delta^2]^{3/2}} d^2 \mathbf{r}'_{\parallel} \times [\nabla \times \boldsymbol{\pi}(\mathbf{r}_{\parallel})] \right\}_{\parallel}, \end{aligned} \quad (\text{S10})$$

having used that  $\nabla g_0(\mathbf{r}, \mathbf{r}') \simeq -(\mathbf{r} - \mathbf{r}')/4\pi|\mathbf{r} - \mathbf{r}'|^3$  for  $\mathbf{r}' \rightarrow \mathbf{r}$  at the second equality, and that  $\hat{\mathbf{n}}$  is orthogonal to  $\mathbf{r}_{\parallel} - \mathbf{r}'_{\parallel}$  for  $\mathbf{r}'_{\parallel} \rightarrow \mathbf{r}_{\parallel}$  at the third equality. The remaining integral can be evaluated over  $\mathbf{r}'_{\parallel} \in \mathbb{R}^2$  rather than over  $\mathbf{r}'_{\parallel} \in \partial\Omega$  (cf. its singular localization as  $\delta \rightarrow 0^+$ ) and equals  $4\pi\hat{\mathbf{n}}$ <sup>¶</sup> so that

$$\begin{aligned} \llbracket \mathbf{E}_{\parallel} \rrbracket &= -\varepsilon_0^{-1} \left\{ \hat{\mathbf{n}} \times [\nabla \times \boldsymbol{\pi}(\mathbf{r}_{\parallel})] \right\}_{\parallel} = -\varepsilon_0^{-1} \left\{ \hat{\mathbf{n}} \times [\nabla \times \boldsymbol{\pi}(\mathbf{r}_{\parallel})\hat{\mathbf{n}}] \right\}_{\parallel} \\ &= -\varepsilon_0^{-1} \left\{ \hat{\mathbf{n}} \times [\nabla \pi(\mathbf{r}_{\parallel})] \times \hat{\mathbf{n}} \right\}_{\parallel} && \text{cf. } \nabla \times (\pi \hat{\mathbf{n}}) = (\nabla \pi) \times \hat{\mathbf{n}} + \pi \nabla \times \hat{\mathbf{n}} = (\nabla \pi) \times \hat{\mathbf{n}} \\ & && \text{since the curl of a normal vector } \hat{\mathbf{n}} \text{ vanishes} \\ &= -\varepsilon_0^{-1} \nabla_{\parallel} \pi(\mathbf{r}_{\parallel}). && \text{cf. } \hat{\mathbf{n}} \times \mathbf{f} \times \hat{\mathbf{n}} = (1 - \hat{\mathbf{n}}\hat{\mathbf{n}}^T)\mathbf{f} = \mathbf{f}_{\parallel} \text{ and } (\mathbf{f}_{\parallel})_{\parallel} = \mathbf{f}_{\parallel} \end{aligned} \quad (\text{S11})$$

Inserting this into Eq. (S4a) then finally yields the self-consistent BC for  $\mathbf{E}_{\parallel}$ , that is, Eq. (S5c).

That the surface dipole density does not change the classical BC for  $B_{\perp}$ , i.e.  $\llbracket B_{\perp} \rrbracket = 0$ , can be derived in much the same way by considering the magnetic dyadic Green function  $\nabla \times \mathbf{G}_0 = \nabla g_0 \times \mathbf{1}$ . The  $\mathbf{B}$ -field due to a current  $\mathbf{J} = -i\omega\pi\delta(\mathbf{r} - \partial\Omega)$  is  $\mathbf{B}(\mathbf{r}) = \int_{\mathbb{R}^3} \nabla g_0(\mathbf{r}, \mathbf{r}') \times \mathbf{J}(\mathbf{r}') d^3 \mathbf{r}' = -i\omega \int_{\partial\Omega} \nabla g_0(\mathbf{r}, \mathbf{r}'_{\parallel}) \times \boldsymbol{\pi}(\mathbf{r}'_{\parallel}) d^2 \mathbf{r}'_{\parallel}$ .<sup>\*\*</sup> Any possible dipole-contributed discontinuity is then equal to (as for  $\llbracket \mathbf{E}_{\parallel} \rrbracket$ , the bulk and in-plane surface current terms do not contribute to any discontinuity)

$$\begin{aligned} \llbracket B_{\perp} \rrbracket &= \lim_{\delta \rightarrow 0^+} B_{\perp}(\mathbf{r}_{\parallel} + \delta \hat{\mathbf{n}}) - B_{\perp}(\mathbf{r}_{\parallel} - \delta \hat{\mathbf{n}}) \\ &= -i\omega \lim_{\delta \rightarrow 0^+} \left\{ \int_{\partial\Omega} [\nabla g_0(\mathbf{r}_{\parallel} + \delta \hat{\mathbf{n}}, \mathbf{r}'_{\parallel}) - \nabla g_0(\mathbf{r}_{\parallel} - \delta \hat{\mathbf{n}}, \mathbf{r}'_{\parallel})] \times \boldsymbol{\pi}(\mathbf{r}') d^2 \mathbf{r}' \right\}_{\perp} \\ &= i\omega \lim_{\delta \rightarrow 0^+} [\hat{\mathbf{n}} \times \boldsymbol{\pi}(\mathbf{r}')]_{\perp} && \text{cf. footnote ¶} \\ &= 0. && \text{cf. } \boldsymbol{\pi} \propto \hat{\mathbf{n}} \text{ and } \hat{\mathbf{n}} \times \hat{\mathbf{n}} = \mathbf{0} \end{aligned} \quad (\text{S12})$$

**Retarded reflection coefficient** Combining the mesoscopic BCs Eqs. (S5) with the macroscopic Maxwell equations, we can immediately verify that we obtain Feibelman's original result for the retarded reflection coefficient of a planar surface [S1; S3; S12]. Specifically, for a TM-polarized wave<sup>††</sup> impinging onto the interface from above, one finds

$$r^{\text{TM}} = \frac{\varepsilon^- \kappa^+ - \varepsilon^+ \kappa^- + (\varepsilon^- - \varepsilon^+)(k_{\parallel}^2 d_{\perp} + \kappa^- \kappa^+ d_{\parallel})}{\varepsilon^- \kappa^+ + \varepsilon^+ \kappa^- - (\varepsilon^- - \varepsilon^+)(k_{\parallel}^2 d_{\perp} - \kappa^- \kappa^+ d_{\parallel})}, \quad (\text{S13})$$

with  $\kappa^{\pm} = \sqrt{k_{\parallel}^2 - \varepsilon^{\pm} k_0^2} = -ik_{\perp}^{\pm}$ . Note that the nonretarded limit of  $r^{\text{TM}}$  differs by a sign from the potential-related reflection coefficient  $r$  in Eq. (S1a): this is a trivial consequence of  $\mathbf{E} = -\nabla\phi$ .

### S3. NUMERICAL IMPLEMENTATION

Here we consider a general electromagnetic scattering problem (as in our experiment) to illustrate the numerical implementation in COMSOL Multiphysics. Other electromagnetic problems can be treated in

<sup>¶</sup> Thus,  $\lim_{\delta \rightarrow 0^+} [\nabla g_0(\mathbf{r}_{\parallel} + \delta \hat{\mathbf{n}}, \mathbf{r}'_{\parallel}) - \nabla g_0(\mathbf{r}_{\parallel} - \delta \hat{\mathbf{n}}, \mathbf{r}'_{\parallel})]$  is in fact a weak representation of the Dirac delta function  $-\delta^2(\mathbf{r}_{\parallel} - \mathbf{r}'_{\parallel})\hat{\mathbf{n}}$ .

<sup>\*\*</sup> For simplicity, we assume  $\mu = 1$  (non-magnetic response,  $\mathbf{H} = \mathbf{B}$ ). Including magnetic response does not change the outcome.

<sup>††</sup> For a TE-polarized wave, the result is  $r^{\text{TE}} = \frac{\kappa^- - \kappa^+ + (\kappa^+)^2(\varepsilon^+ - \varepsilon^-)d_{\parallel}}{\kappa^- + \kappa^+ + (\kappa^+)^2(\varepsilon^+ - \varepsilon^-)d_{\parallel}}$  [S3], i.e. not impacted by  $d_{\perp}$ .

a similar manner.

The scattering formulation of Maxwell's equations yields

$$\nabla \times \mu^{-1} \nabla \times \mathbf{E}_{\text{sca}} - \varepsilon(\mathbf{r}, \omega) k^2 \mathbf{E}_{\text{sca}} = \Delta \varepsilon(\mathbf{r}, \omega) k^2 \mathbf{E}_{\text{inc}}, \quad (\text{S14})$$

where  $k = \omega/c$ ,  $\mathbf{E}_{\text{inc}}$  is the incident field,  $\mathbf{E}_{\text{sca}}$  is the scattered field, and  $\Delta \varepsilon(\mathbf{r}) = \varepsilon(\mathbf{r}) - \varepsilon_{\text{bg}}(\mathbf{r})$  is the permittivity contrast between the scattering object and its background (vanishes outside the scatterer).

Eq. (S14) and Eqs. (S5) constitute the full ingredients for numerically solving our scattering problem. Specifically, in our gap plasmon nanoresonator structures, the incident field  $\mathbf{E}_{\text{inc}}$  in Eq. (S14) is defined as the summation of the incident plane waves and their reflected fields from the substrate. Using the TM polarization for example,

$$\mathbf{E}_{\text{inc, TM}} = E_0 \left[ (\hat{\rho} \cos \theta + \hat{\mathbf{z}} \sin \theta) e^{ik_z z + ik_\rho \rho} + r_{\text{TM}} (-\hat{\rho} \cos \theta + \hat{\mathbf{z}} \sin \theta) e^{-ik_z z + ik_\rho \rho} \right], \quad (\text{S15})$$

where  $\theta$  is the incident angle and  $r_{\text{TM}}$  is the (Feibelman-corrected) TM reflection coefficient (Eq. S13). Notably, the nonclassical correction to  $r_{\text{TM}}$  is small  $\sim k_0 d_{\perp, \parallel}$ . We exploit the structure's rotational symmetry by decomposing the incident plane waves in cylindrical harmonics [S13] which allows us to calculate the scattering response for each azimuthal index  $m$  separately. This reduces the dimensionality of the computational problem from three to two, allowing significant reductions in computational time and memory requirements. As our focus is on the lowest order (1, 1) (denotes the radial and azimuthal index number respectively [S14]) resonance, we restrict our considerations to its  $m = 1$  channel.

Implementation wise, the master equation Eq. (S14) is incorporated via weak-form integrals. For the nonclassical BCs [Eqs. (S5)], only two of them [Eqs. (S5c) and (S5a)] are needed to uniquely and completely define the computation. In principle, the boundary conditions Eqs. (S5) can be straightforwardly incorporated by point-wise or weak constraints. However, numerical instability may arise due to the derivative form of Eq. (S5c).

As an alternative, we develop a numerical stable approach to implement those nonclassical BCs. The  $d_{\parallel}$  contribution [Eq. (S5a)] can be incorporated via a surface current term  $\mathbf{K}(\mathbf{r}) = id_{\parallel} \omega \llbracket \mathbf{D}_{\parallel} \rrbracket$ . Specifically for the  $d_{\perp}$  contribution [Eq. (S5c)], we describe below the auxiliary potential method employing its integral form for better numerical stability.

For the scattered field, Eq. (S5c) can be rewritten as

$$\mathbf{E}_{\text{sca}} = \mathbf{E}_{\text{sca}}^c + \nabla \psi, \quad (\text{S16})$$

where  $\mathbf{E}_{\text{sca}}^c$  is the continuous classical scattered field, the scalar auxiliary potential  $\psi$  defined on the boundary  $\partial\Omega$  is given by

$$\psi|_{\partial\Omega}^{\pm} = \mp d_{\perp} \llbracket E_{\perp} \rrbracket. \quad (\text{S17})$$

The potential needs to change sign depending on whether it is defined on the “+” or “−” side of the boundary. Plugging Eq. (S16) into Eq. (S14) yields

$$\nabla \times \mu^{-1} \nabla \times \mathbf{E}_{\text{sca}} - \varepsilon(\mathbf{r}, \omega) k^2 \mathbf{E}_{\text{sca}} = \Delta \varepsilon(\mathbf{r}, \omega) k^2 \mathbf{E}_{\text{inc}} + \varepsilon(\mathbf{r}, \omega) k^2 \nabla \psi. \quad (\text{S18})$$

where the nonclassical contribution (last term on the right-hand side) is implemented via weak-form integrals.

#### S4. QUASI-NORMAL-MODE PERTURBATION THEORY

##### A. Perturbation theory framework

Classically, the electromagnetic resonant eigenfrequency  $\tilde{\omega}$  and eigenfield  $\tilde{\mathbf{E}}$  of a general geometry satisfies the following master equation [ $(\mathbf{r}, \tilde{\omega})$ -dependence implicit]

$$\nabla \times \mu^{-1} \nabla \times \tilde{\mathbf{E}} - \varepsilon \frac{\tilde{\omega}^2}{c^2} \tilde{\mathbf{E}} = 0. \quad (\text{S19})$$

For open resonators with radiative and potentially absorptive losses,  $\tilde{\omega}$  is complex-valued and the outgoing-wave boundary condition is imposed. Hereafter we denote the classical non-perturbed frequencies and fields as  $\tilde{\omega}^{(0)}$  and  $\tilde{\mathbf{E}}^{(0)}$  (throughout, the tilde notation indicates the QNM eigenfrequencies and eigenfields).

Under the QNM framework, eigenfields are normalized under the convention that

$$\int_{\mathbb{R}^3} \left[ \tilde{\mathbf{E}} \cdot \frac{\partial(\omega\epsilon)}{\partial\omega} \Big|_{\tilde{\omega}} \tilde{\mathbf{E}} - \tilde{\mathbf{H}} \cdot \frac{\partial(\omega\mu)}{\partial\omega} \Big|_{\tilde{\omega}} \tilde{\mathbf{H}} \right] d^3\mathbf{r} = 1, \quad (\text{S20})$$

where  $\mathbb{R}^3$  in practice includes both physical and perfectly-matched-layer domains [S15].

Next we “turn on” the nonclassical perturbation, i.e. the surface polarization  $\mathbf{P}_s(d_\perp, d_\parallel; \mathbf{E}) \equiv \boldsymbol{\pi} + i\omega^{-1}\mathbf{K}$ . Evidently, the nonclassical surface polarization is a functional of  $d$ -parameters and the nonclassical eigenfield  $\tilde{\mathbf{E}}$ . The nonclassical master equation naturally emerges as

$$\nabla \times \mu^{-1} \nabla \times \tilde{\mathbf{E}} - \epsilon \frac{\tilde{\omega}^2}{c^2} \tilde{\mathbf{E}} - \frac{\tilde{\omega}^2}{c^2} \mathbf{P}_s(d_\perp, d_\parallel; \tilde{\mathbf{E}}) \delta(\mathbf{r} - \partial\Omega) = 0. \quad (\text{S21})$$

Within first-order perturbation,  $\tilde{\omega} = \tilde{\omega}^{(0)} + \tilde{\omega}^{(1)} + \mathcal{O}[(\tilde{\omega} - \tilde{\omega}^{(0)})^2]$ . The first-order correction,  $\tilde{\omega}^{(1)}$ , is given by an inner product between the unperturbed eigenfield and the perturbing polarization [S16]. Specifically, the nonclassical surface correction can be calculated by a surface integral runs over all interfaces

$$\tilde{\omega}^{(1)} = -\tilde{\omega}^{(0)} \int_{\partial\Omega} \tilde{\mathbf{E}}^{(0)} \cdot \tilde{\mathbf{P}}_s^{(0)} d^2\mathbf{r}, \quad (\text{S22})$$

with  $\tilde{\mathbf{P}}_s^{(0)} \equiv \mathbf{P}_s(d_\perp, d_\parallel; \tilde{\mathbf{E}}^{(0)})$ . In contrast to conventional perturbation theory, an unconjugated inner product is used between the ground-state and perturbing components (and in the normalization condition), reflecting the non-Hermitian nature of the QNM eigenproblem [S15].

The nonclassical surface polarization  $\mathbf{P}_s$  requires further specifications—in terms of which medium it placed—to render Eq. (S21) consistent with the generalized boundary conditions, Eqs. (S5). To illustrate such necessity, we observe that, if  $\mathbf{P}_s$  is simply chosen to place in metal or dielectric sides of metal-dielectric interfaces, the generalized boundary condition of  $\mathbf{E}_\parallel$  shall be modified to  $[\mathbf{E}_\parallel] = -d_\perp \nabla_\parallel [E_\perp] / \epsilon_b$ , where the extra term  $\epsilon_b$  represents the permittivity of background media in which  $\mathbf{P}_s$  is embedded. This modification comes from the fact that, when defining the surface polarization  $\boldsymbol{\pi}$  and current  $\mathbf{K}$  in relation with  $d_\perp$  and  $d_\parallel$ , respectively, we choose vacuum as background, in which  $\boldsymbol{\pi}$  and  $\mathbf{K}$  radiate, see Eq. S6. Respecting this prerequisite, we, thus, introduce an infinitely thin vacuum layer separating the metal and the dielectric, and  $\mathbf{P}_s$  is placed on this vacuum layer; in this way, it could be examined that the generalized boundary condition of Eq. (S5c) is restored. Alternatively, instead of introducing an auxiliary vacuum layer, one can multiply  $\boldsymbol{\pi}$  defined in Eq. (S4a) by factor  $\epsilon_b$  to compensate the screening modification. Both two approaches produce same results. Below, to derive the QNM perturbation formalism, we choose the former approach to set  $\mathbf{P}_s$ .

Substituting Eqs. (S4a) and (S4b) into Eq. (S22) then produces Eq. (2), i.e.  $\tilde{\omega}^{(1)} = \tilde{\omega}^{(0)} \sum_\tau \kappa_\perp^\tau d_\perp^\tau + \kappa_\parallel^\tau d_\parallel^\tau$  with the perturbation strengths  $\kappa_\perp$  and  $\kappa_\parallel$  (in units of inverse length) introduced in the main text and restated below:

$$\kappa_\perp^\tau \equiv - \int_{\partial\Omega^\tau} \tilde{D}_\perp^{(0)} [\tilde{E}_\perp^{(0)}] d^2\mathbf{r}, \quad \kappa_\parallel^\tau \equiv \int_{\partial\Omega^\tau} \tilde{\mathbf{E}}_\parallel^{(0)} \cdot [\tilde{\mathbf{D}}_\parallel^{(0)}] d^2\mathbf{r}. \quad (\text{S23a})$$

Here,  $\tau$  runs over all material interfaces such that  $\bigcup_\tau \partial\Omega^\tau = \partial\Omega$ .

## B. Perturbation result in the cylindrical coordinates

Next, we describe some unique considerations necessary to facilitate the perturbation calculations in cylindrical coordinates. Given the axial symmetry of the experimental nanodisk structure, the resonance modes'  $\mathbf{E}$ -field assume the form  $\tilde{\mathbf{E}}_m(\mathbf{r}, \tilde{\omega}) = \tilde{\mathbf{E}}_m(\rho, z) e^{im\phi} e^{-i\tilde{\omega}t}$ , expressed in cylindrical coordinates  $(\rho, \phi, z)$  and with  $m = 0, \pm 1, \pm 2, \dots$  (the modes are also index by a radial quantization number  $n$ ; it is suppressed here for clarity).

For nonzero  $m$ , Eq. (S20) suggests a vanishing normalization integral. For these azimuthally varying modes, the normalization condition is revised to

$$\int_{\mathbb{R}^3} \left[ \tilde{\mathbf{E}}_{-m} \cdot \frac{\partial(\omega\epsilon)}{\partial\omega} \Big|_{\tilde{\omega}} \tilde{\mathbf{E}}_m - \tilde{\mathbf{H}}_{-m} \cdot \frac{\partial(\omega\mu)}{\partial\omega} \Big|_{\tilde{\omega}} \tilde{\mathbf{H}}_m \right] d^3\mathbf{r} = 1, \quad (\text{S24})$$

where  $\tilde{\mathbf{E}}_{-m} = [\tilde{\mathbf{E}}_m \cdot \hat{\rho}, -\tilde{\mathbf{E}}_m \cdot \hat{\phi}, \tilde{\mathbf{E}}_m \cdot \hat{z}]$  and  $\tilde{\mathbf{H}}_{-m} = [-\tilde{\mathbf{H}}_m \cdot \hat{\rho}, \tilde{\mathbf{H}}_m \cdot \hat{\phi}, -\tilde{\mathbf{H}}_m \cdot \hat{z}]$ : this produces a  $\phi$ -invariant integrand and a nonzero normalization integral.

The perturbation strengths  $\kappa_{\perp,\parallel}^\tau$  are similarly revised:

$$\kappa_\perp^\tau \equiv - \int_{\partial\Omega^\tau} \tilde{D}_{\perp,-m}^{(0)} \llbracket \tilde{E}_{\perp,m}^{(0)} \rrbracket d^2\mathbf{r}, \quad \kappa_\parallel^\tau \equiv \int_{\partial\Omega^\tau} \tilde{\mathbf{E}}_{\parallel,-m}^{(0)} \cdot \llbracket \tilde{\mathbf{D}}_{\parallel,m}^{(0)} \rrbracket d^2\mathbf{r}. \quad (\text{S25})$$

These revisions are necessary due to the degeneracy of  $m = \pm|m|$  ( $\neq 0$ ) modes in the axially symmetric structure: the perturbation expressions in Eqs. (S24)–(S25) are derived under the framework of non-degenerate perturbation theory, and so are not directly applicable to the degenerate case. In this doubly-degenerate case, non-degenerate perturbation theory produces a  $2 \times 2$  matrix-form: the diagonal terms vanish and the off-diagonal terms [i.e. Eqs. (S24)–(S25)] remain.

### C. Perturbation strength comparison

Based on Eqs. (S22)–(S23), the nonclassical corrections can be reformulated as [shown in Eq. (2)]

$$\tilde{\omega}^{(1)} \equiv \tilde{\omega}^{(0)} \sum_\tau \kappa_\perp^\tau d_\perp^\tau + \kappa_\parallel^\tau d_\parallel^\tau, \quad (\text{S26})$$

where  $\tau \in \{\text{Au-AIO}_x, \text{Au-air}\}$  for our Au–Au setup. The summation gives rise to four discrete corrections on the Au–air and Au–AIO<sub>x</sub> interfaces in our structure.

Figure S2a (same as Fig. 3a) shows the magnitude of the perturbation prefactors  $|\kappa_\alpha^\tau|$  ( $\alpha \in \{\perp, \parallel\}$ ) as a function of gap size for the film-coupled Au nanodisk. For our experimentally considered gap sizes, we find that  $\kappa_\parallel^\tau$  are negligible compared to  $|\kappa_\perp^{\text{Au-AIO}_x}|$  [about one and two order(s) of magnitude smaller for big ( $\approx 8$  nm) and small ( $\approx 1$  nm) gaps, respectively]. The sharp difference in perturbation strengths is a consequence of the highly confined electric field (in the gap) being mostly in the surface normal direction.

For the perturbation strengths of the two  $d_\perp$  corrections,  $|\kappa_\perp^{\text{Au-AIO}_x}|$  is about one magnitude larger than  $|\kappa_\perp^{\text{Au-air}}|$  for smaller gaps ( $\lesssim 4$  nm), and remains larger but comparable for bigger gaps ( $\gtrsim 6$  nm). On the other hand, due to screening from the dielectric cladding (Sec. S16), the magnitude of the  $d$  parameters of a Au–dielectric interface is larger than that of a Au–vacuum(air) interface. We note that a recent work [S12] reports a similar conclusion for Ag in its density-function-theory calculation.

Based on the aforementioned complementary arguments for the relative magnitude of  $\kappa_\alpha^\tau$  and  $d_\alpha^\tau$  respectively, we approximate Eq. (S26) by

$$\tilde{\omega}^{(1)} \approx \tilde{\omega}^{(0)} \kappa_\perp^{\text{Au-AIO}_x} d_\perp^{\text{Au-AIO}_x}. \quad (\text{S27})$$

Applying Eq. (S27) to the experimental spectral shift and broadening, we are able to extract  $d_\perp^{\text{Au-AIO}_x}$  explicitly from the measurements, as shown in Fig. 3a,b.

In our analysis, the perturbing term is eigenvalue-dependent (i.e.  $\tilde{\mathbf{P}}_s^{(0)}$  depends on  $\tilde{\omega}$ ) and therefore the entire perturbation becomes dispersive/nonlinear. Therefore, the perturbation center should be judiciously chosen. For  $\text{Re } d_\perp^{\text{Au-AIO}_x}$  (which is quite dispersionless; see Fig. 3a), the classical frequency is treated as the perturbation center (i.e. a simple pole approximation). For  $\text{Im } d_\perp^{\text{Au-AIO}_x}$ , the nonclassical frequency is treated as the perturbation center to count for its strong frequency-dispersion (see Fig. 3b). In other words, the spectral shift (Re  $d$  contribution) and broadening (Im  $d$  contribution) are ‘turned on’ successively (not simultaneously) in order to reduce the second-order  $\mathcal{O}[(\tilde{\omega} - \tilde{\omega}^{(0)})^2]$  error in the perturbation analysis.

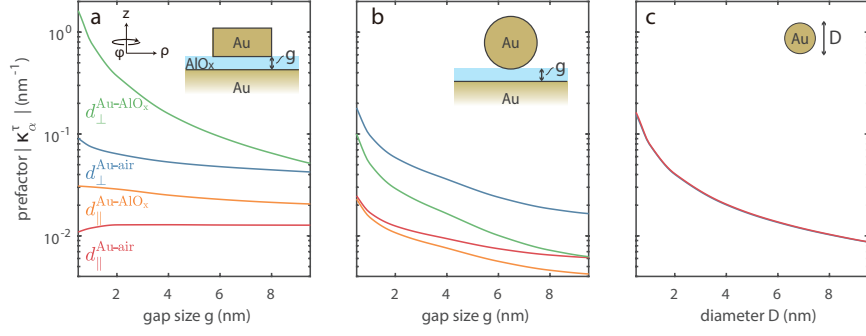

**Figure S2. Nonclassical perturbation strength comparison of various Au structures.** **a.** Au disk (diameter, 70.4 nm; height, 31 nm) on Au substrate. **b.** Au sphere (diameter, 70 nm) on Au substrate. **c.** Au sphere in vacuum; its  $d_{\perp}$  and  $d_{\parallel}$  perturbation strength are the same in magnitude, but of opposite signs.

#### D. Structural dependence of the spectral shift

In our experiment we observe large nonclassical corrections in the film-coupled Au disk structures (Fig. 3). The observed nonclassical corrections are much larger than those in standalone nanospheres [S17] or film-coupled nanospheres [S18] for similar separations (or particle sizes). Such contrast highlights the structural dependence of the nonclassical corrections, as confirmed by our perturbation analysis in Fig. S2. We find that a film-coupled nanosphere in the retarded regime and a standalone nanosphere in the nonretarded regime exhibit similar maximal perturbation strengths (Fig. S2b,c). In contrast, the perturbation strength of our experimental Au–Au nanodisk structure is about one order of magnitude larger (Fig. S2a).

#### S5. SAMPLE FABRICATION

Figure S3 shows the fabrication flow. The nanoresonators consisted of three main components: the bottom Au reflector, the middle  $\text{AlO}_x$  spacer, and the top Au/Al/Si nanodisk.

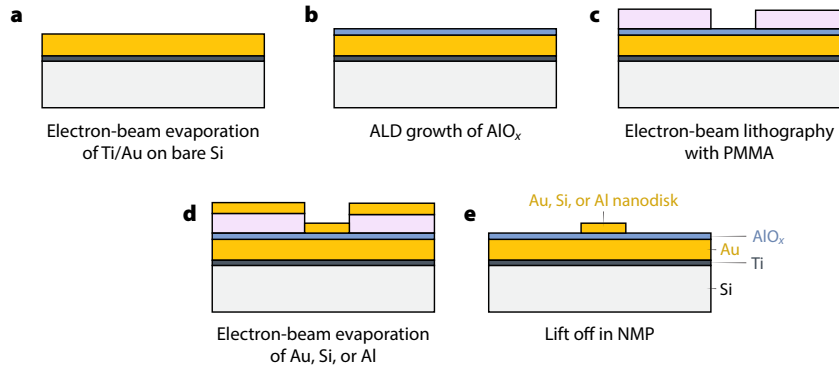

**Figure S3. Fabrication process for the plasmonic resonators.** **a.** Electron evaporation of 10 nm Ti and 60 nm Au on a bare Si wafer. **b.** Atomic layer deposition of  $\text{AlO}_x$  at 120 °C with 5, 10, 20, 40, 60, and 80 cycles. **c.** Patterning of the nanodisks with PMMA in a 125 keV electron-beam lithography system. **d.** Electron-beam evaporation of 40 nm of Au/Si/Al without adhesion layer. **e.** Lift-off of the evaporated materials in 60 °C NMP.

The bottom Au reflector was fabricated by depositing 10 nm Ti followed by 60 nm Au on a 4-inch Si wafer using electron-beam-induced evaporation at a rate of  $1 \text{ \AA s}^{-1}$  with a vacuum pressure of  $\approx 1 \times 10^{-6}$  Torr. The 4-inch wafer was then cleaved into smaller pieces as the base substrates for subsequent fabrication steps.

The  $\text{AlO}_x$  spacer was grown on the Au-coated substrate using atomic layer deposition (ALD) at 120 °C

with a base pressure of 0.214 Torr. The substrate was cleaned using  $O_2$  plasma ashing at 100 W for 2 min before the deposition. Each deposition cycle consisted of a 15 ms pulsing of trimethylaluminum (TMA) and 20 ms pulsing of standard water ( $H_2O$ ) with a 8 s wait time in between. Six different deposition cycles were chosen (5, 10, 20, 40, 60, and 80), where each cycle was expected to deposit a single layer of  $AlO_x$  with a thickness of  $\approx 1$  Å. Three preconditioning buffer cycles were added before the actual cycles started.

The nanodisks were then patterned on top of the  $AlO_x$  spacer via electron-beam lithography (EBL). A positive-tone electron-beam resist, poly(methyl methacrylate) (MircoChem 950PMMA A4), was spin coated on the substrate at 4 krpm and baked at 180 °C for 2 min. The thickness of the PMMA was measured to be 192 nm using a reflectometer (Filmetrics F20). A 125 kV electron-beam lithography system (Elionix F-125) was used to expose the PMMA with a beam current of 1 nA and dose of  $3000 \mu C cm^{-2}$ . The exposed PMMA was developed in MIBK:IPA (1:3) at 0 °C for 90 s, followed by a 30 s IPA dip and  $N_2$  blow dry. Au, Al, or Si films with a nominal thickness of 40 nm were then deposited by electron-beam-induced evaporation. To avoid plasmon damping, no adhesion layer was used. After evaporation, the resist was lifted-off in *n*-methyl-2-pyrrolidone (NMP) at 65 °C for approximately 60 min, followed by a rinse in IPA and  $N_2$  blow dry. The actual thicknesses of the evaporated films were measured using an AFM on micrometer-size dummy structures on the samples and found to be 31.0 nm for Au, 40.4 nm for Al, and 41.7 nm for Si.

In total, 18 chips were fabricated: 3 materials (Au, Al, Si), each with 6 different  $AlO_x$  thicknesses. Each chip had multiple blocks of nanodisk with varying diameters. Each block consisted of  $51 \times 51$  nanodisk array, and the spacing between the nanodisks was kept at 2  $\mu m$  to minimize cross-talk.

## S6. SURFACE ROUGHNESS

The surface roughness of the ALD  $AlO_x$  and evaporated Au film was measured using an atomic force microscope (Nanoscope V with Dimension 3100). Figure S4 shows an AFM image of a 40-cycle-ALD  $AlO_x$  chip after all fabrication processes. The root mean square (rms) roughness was 0.578 nm and the correlation length of the grain was  $\approx 50$  nm. On a 10-cycle-ALD  $AlO_x$  chip, we measured an rms roughness of 0.677 nm. This slight increase of rms roughness agrees with the fact that ALD conformally coat the substrate and smooths the surface.

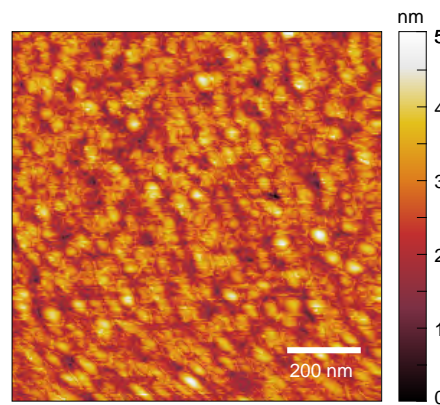

**Figure S4. Surface roughness of an ALD  $AlO_x$  coated Au film.** The AFM measurement was performed on a 40-cycle ALD  $AlO_x$  coated Au film. The rms surface roughness was 578 pm.

## S7. NANODISK SIZE DISTRIBUTION

Figure S5 shows the collected size statistics of the Au nanodisks. For each nominal size, 100 nanodisks were imaged using scanning electron microscope. These images were processed using a Python program and the area of each nanodisk was extracted. The diameter was then estimated as  $D = 2 \sqrt{A/\pi}$ , where  $A$  is the area. This approach compensates for the perimeter roughness and irregularity of individual nanodisks.

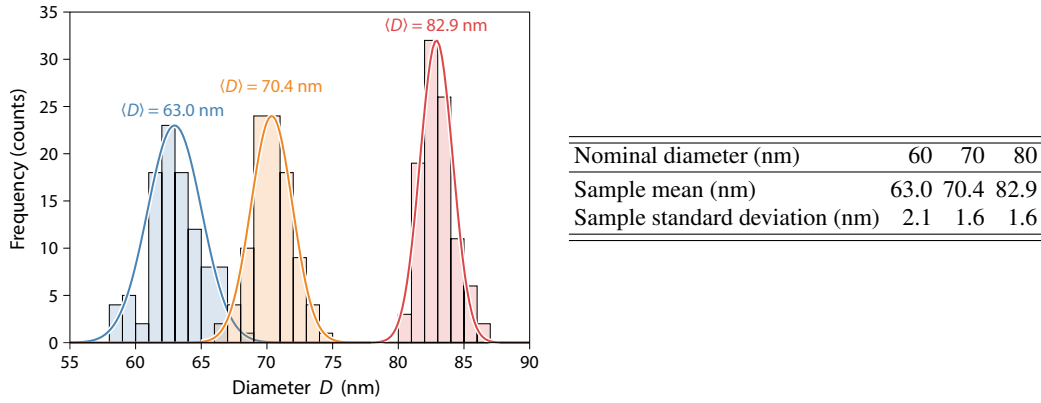

**Figure S5. Size statistics of fabricated Au nanodisks.** Collected histograms, including Gaussian distribution fits (left) and distribution statistics (right).

Similarly, the size distribution of Al nanodisks were calculated and shown in Table I. For each nominal size,  $\geq 20$  nanodisks were imaged.

| Nominal diameter (nm)          | 60   | 70   | 80   |
|--------------------------------|------|------|------|
| Sample mean (nm)               | 62.7 | 70.5 | 83.5 |
| Sample standard deviation (nm) | 2.9  | 2.3  | 2.4  |

Table I **Size statistics of fabricated Al nanodisks.**

Due to the low imaging contrast of the Si nanodisks, we were not able to use the image processing program. Instead, we measured the nanodisk diameters manually in ImageJ (a free image processing software). For each nominal size, we measured  $\geq 20$  nanodisks, and calculated the mean and standard deviation of the size distributions as shown in Table II.

| Nominal diameter (nm)          | 80   | 90   | 100   | 110   | 120   | 130   | 140   |
|--------------------------------|------|------|-------|-------|-------|-------|-------|
| Sample mean (nm)               | 84.3 | 92.9 | 104.4 | 113.1 | 124.0 | 138.1 | 145.9 |
| Sample standard deviation (nm) | 3.9  | 2.8  | 2.2   | 2.8   | 4.0   | 3.7   | 2.3   |

Table II **Size statistics of fabricated Si nanodisks.**

## S8. CROSS-SECTIONAL TRANSMISSION ELECTRON MICROGRAPH

Figure S6 shows the annular dark-field scanning transmission electron microscope (ADF-STEM) images of a Au–AlO<sub>x</sub>–Au stack from an Au-particle chip with 4 nm AlO<sub>x</sub> spacer. To prepare the sample, a micrometer-size dummy structure was fabricated on the same chip that was used for dark-field scattering measurement, and the top of the structure was protected by a 60-nm-thick hydrogen silsesquioxane (HSQ) layer. A cross-sectional sample was cut and lifted-out from this dummy structure using a 30-kV gallium-focused-ion-beam (Thermo Scientific Helios Nanolab 600). The sample was welded onto a copper Omniprobe lift-out grid and thinned down to  $\approx 100$  nm. The images of this sample in figure S6 were taken using a JEOL 2010F TEM-STEM operating at 200 kV.

## S9. ELLIPSOMETRY

The bulk permittivities of the evaporated Au, Al, and Si used in the experiments were measured using a variable-angle spectroscopic ellipsometer (J.A. Woolam Co., Inc., benchtop XLS-100 UV-VIS continuous spectroscopic ellipsometer and WVASE32 software).

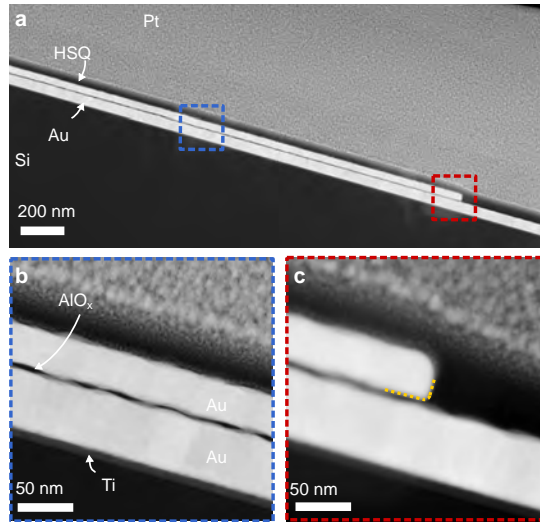

**Figure S6. Cross-sectional transmission electron micrograph of the  $\text{AlO}_x$  spacer.** **a.** The sample was cut from a micrometer-size dummy structure fabricated on the same chip that was used for dark field scattering measurement. From bottom to top, the stack contains Si, Ti, Au,  $\text{AlO}_x$ , Au, HSQ, and Pt. The HSQ and Pt were used to protect the sample from ion beam damaging during FIB. **b.** Zoomed view on the  $\text{AlO}_x$  gap. The thickness of the  $\text{AlO}_x$  was  $\approx 4$  nm. **c.** The edge of the lift-off Au structure, showing a radius of curvature of  $\approx 2$  nm on the bottom edge.

The bare Au sample for ellipsometry measurement was prepared by evaporating 10 nm Ti followed by 60 nm Au (nominal thicknesses) on a 4-inch Si wafer. The wafer was cleaved into smaller pieces as the base substrates for other samples. We then evaporated 40 nm Si and 40 nm Al on the Au-coated substrates for measuring the permittivities of Si and Al, respectively.

Spectroscopic scans were performed at the  $70^\circ$  relative to the surface normal of the samples. We verified that the measured permittivities were consistent across various incident angles ( $60-80^\circ$ ). Ellipsometry data were analyzed using multi-layer models and the surface roughness (measured by AFM) was taken into account via the Bruggeman effective medium theory [S19]. The measured permittivities for the three materials are shown in Fig. S7 and are used for our subsequent measurements and theoretical calculations. Specifically for the permittivities of Au, our results agree well with the Johnson–Christy data [S20] in the visible regime. Therefore, we adopted the Johnson–Christy data for energies below 1.24 eV (equivalently, for wavelengths above 1000 nm, corresponding to the cut-off wavelength of our ellipsometer).

For Si and Al evaporated films, an extra native oxide layer was taken into account to measure their native oxide thickness in ambient conditions. We found the native oxide thickness of the Si film  $\approx 1.5$  nm as of measurement. The native oxide thickness of the Al film is  $\approx 4$  nm, consistent with previous studies (e.g. [S21]).

Ellipsometry was also used to measure the thicknesses and permittivities of the ALD-deposited  $\text{AlO}_x$  gap on the Au substrate (permittivities experimentally determined; see Fig. S7a). The ellipsometric data were collected with the same approach as described for bulk permittivities. The thicknesses  $g$  and the  $\text{AlO}_x$  refractive indices (modelled by the Cauchy dispersion:  $n(\lambda) = A + B/\lambda^2$ , where  $\lambda$  is in  $\mu\text{m}$ ) are fitted to achieve minimal root-mean-square errors.

The measured gap size as a function of deposition cycle is shown in Fig. S8a. The linear fitting yields a deposition rate of  $0.97 \text{ \AA}$ , consistent with the  $\approx 1 \text{ \AA/cycle}$  rate reported in literature [S18; S22; S23]. The  $6.49 \text{ \AA}$  offset may be due to the extra preconditioning purging cycles in the ALD process.

The Cauchy model parameters  $A$  and  $B$ , as well as their exponential fittings are shown in Figs. S8b and S8c. We find that the dispersion-less part (coefficient  $A$ ) of the refractive index decreases for smaller gap sizes and approaches the bulk index for larger gaps. This gap-dependent refractive index of ultrathin  $\text{AlO}_x$  ALD layers has been observed elsewhere [S23] and may be explained by the substrate lattice mismatch, interfacial contaminants, or the saturation of the phase transition layer as deposition cycles increase. Similar thickness-dependent permittivity was also reported in other ALD-grown thin-films [S24]. The

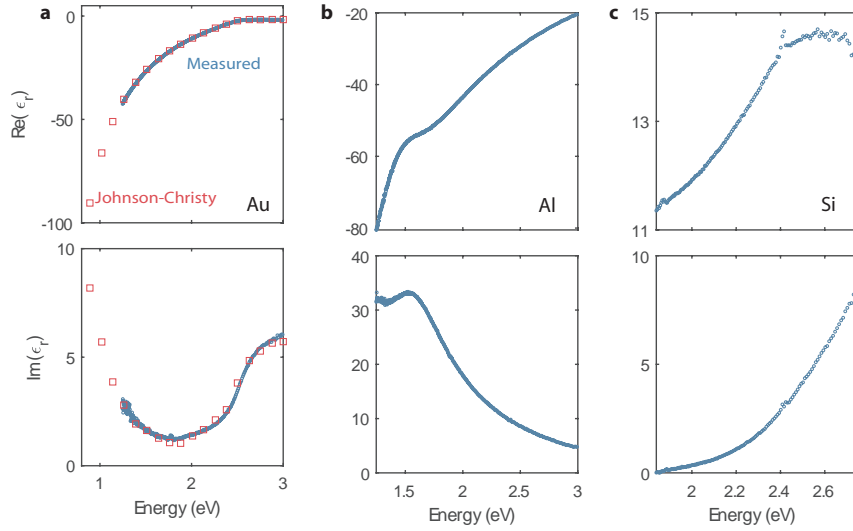

**Figure S7. Ellipsometric measurement of bulk permittivities. a. Au, b. Al, and c. Si.**

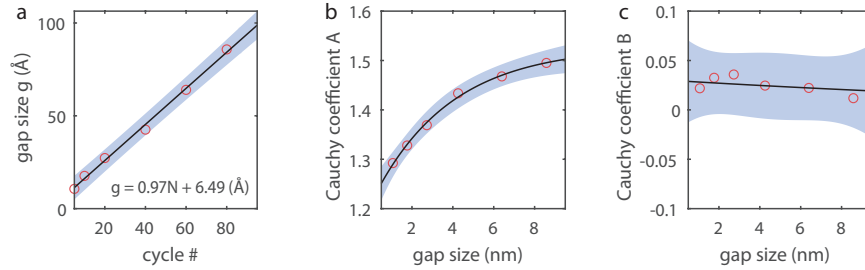

**Figure S8. Ellipsometric measurement of  $\text{AlO}_x$  thickness and refractive indices. a.** Measured thicknesses as a function of deposition cycles (dots) and the linear fitting (line and inset equation) with 95% confidence interval (shading). **b,c.** Measured Cauchy coefficients A and B (dots) and the exponential fitting ( $y = ae^{-bx} + c$ ) with 95% confidence interval.

dispersive part (coefficient  $B$ ) of the refractive index slightly increases for smaller gaps (Fig. S8c). The  $\text{AlO}_x$  refractive indices for different gap sizes are shown in Fig. 3d.

## S10. DARK FIELD SCATTERING MEASUREMENT

We built a table-top optical setup for the dark-field (DF) scattering measurement, as shown in Fig. 2a. Collimated broadband visible and infrared lamp (Oshio Halogen EKE and Kahoku OSL2BIR) illumination (path shown in yellow) is used as the source for the setup. To create dark field illumination, a beam block with diameter  $\approx 2$  cm blocks the center of the beam. An objective lens (Nikon, TU Plan ELWD, 100 $\times$  magnification, 0.8 NA) focuses lamp light onto the mounted sample. Light scattered from the sample (path shown in gray) is collected with the same objective and goes through another magnification element (Optem Zoom 70XL, 7:1 zoom) with tunable focus and magnification. The system thus provides a total of 700 $\times$ 700 maximal magnification, at which the scattering signal of an ensemble of  $\lesssim 100$  nanoparticles is collected. With the flip mirror, the scattered light is subsequently directed into either a CMOS camera (AmScope MU1000) for imaging or a spectrometer (Princeton Instrument Action SP-2360-2300i). Measured counts were normalized to the reflection of a Ag mirror placed at the sample position to obtain the scattering cross-section.

### S11. IMPACT OF SURFACE ROUGHNESS ON OPTICAL RESPONSE

In this section we numerically show that the surface roughness introduces negligible error to the resonant eigenvalue on the complex plane, since the ALD process [S22] is highly conformal.

Fig. S9 illustrates the cross-sectional view ( $\rho, z$ ) of the Au nanoresonator on the Au substrate without (Fig. S9a) and with (Fig. S9b) surface roughness taken into account, respectively. The roughness of the evaporated Au substrate is modeled by spatial sinusoidal variations. Since the fabrication process is conformal, the variation is inherited by the subsequent ALD gap layer and the nanoresonator. The periodicity  $\kappa$  and the peak-to-peak value  $\delta_{pp} = 2\sqrt{2}\delta_{rms}$  of the spatial variation are taken from the experimental (AFM) measurement of the grain size  $\approx 50$  nm and the surface roughness  $\delta_{rms} \approx 0.6$  nm.

Fig. S9c shows the negligible influence of measured surface roughness on the eigenfrequency of the nanoresonator. The resonant frequency drift is  $< 1.2\%$  for all possible random configurations (parameterized by the variable  $\theta$ ) of our structure due to surface roughness. We also verified that this conclusion also holds for Al and Si nanoresonators.

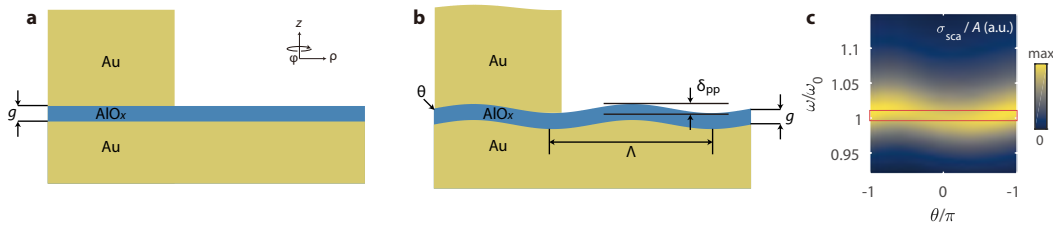

**Figure S9. Analysis of the surface roughness dependence on the optical responses of ALD-fabricated gap plasmonic nanoresonators.** **a,b.** Schematic illustration of the roughness-free **(a)** and conformal surface roughness model **(b)**. The roughness of the evaporated Au substrate is modeled by spatial sinusoidal variations. The gap size, sinusoidal periodicity and peak-to-peak amplitude are denoted by  $g$ ,  $\kappa$ , and  $\delta_{pp}$ , respectively. The position of the center of the nanoresonator with regard to the spatial variation introduces another degree of freedom, the initial ‘phase’ factor  $\theta$ . **c.** Roughness-induced shifts of the resonant frequency and width are negligible given the smoothness level of our fabrication process. The red box denotes the minor resonant frequency shift range ( $< 1.2\%$ ) for all possible random structural variations (i.e.,  $\theta \in [-\pi, \pi]$ ).

### S12. DATA ANALYSIS

#### A. Complex resonant frequency extraction from experiment

As stated in Section S10, our measurement system captures the scattering from  $\lesssim 100$  nanoparticles. Therefore, to obtain the complex resonant frequency of a single nanoresonator, we need to take into account another broadening mechanism, the inhomogeneity of the particle sizes (see Sec. S7). As illustrated in Fig. S10a, the measured spectra are Voigt profiles [S25], i.e. the convolution of the co-centered Lorentzian profile of the resonance and the Gaussian distribution of the particle size

$$V(\omega; \sigma_\omega, \gamma) = \int_{-\infty}^{\infty} G(\omega'; \sigma_\omega) L(\omega - \omega'; \gamma) d\omega', \quad (\text{S28})$$

where  $V$ ,  $G$ , and  $L$  are Voigt, Gaussian, and Lorentzian profiles, respectively.  $\sigma_\omega$  is the Gaussian standard deviation and  $\gamma = \text{Im } \tilde{\omega}$  is the Lorentzian half-linewidth.

We extract the complex resonant frequency  $\tilde{\omega}$  in the following manner. The measured spectra  $S(\omega)$  is treated as the summation of the Voigt profile  $V(\omega; \sigma_\omega, \gamma)$  and the noise background  $N(\omega)$ :

$$S(\omega) = V(\omega; \sigma_\omega, \gamma) + N(\omega). \quad (\text{S29})$$

Here the noise background  $N(\omega)$  is modeled by polynomials with order  $\leq 2$ . The spectral Gaussian standard deviation  $\sigma_\omega$  is measured experimentally. We first obtain the particle diameter standard deviation

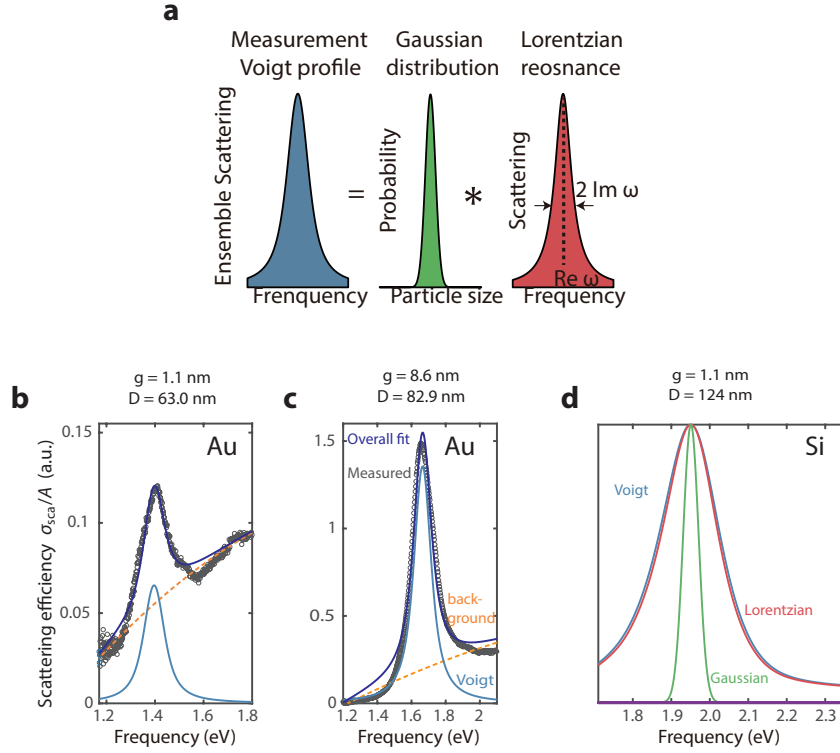

**Figure S10. Data analysis.** **a.** Schematic for the extraction of the complex resonant frequency from the measurement. The convolution of the Gaussian size distribution and the single-particle Lorentzian resonance spectra yields the measured Voigt profile. **b,c.** Fitting the measured scattering of Au nanodisks with a Voigt profile and noise background [see Eq. (S29)]. Two extreme cases are shown—smallest disk diameter on thinnest gap (**b**) and largest disk on thickest gap (**c**). **d.** Resonance broadening (blue) on the simulated nonclassical single-particle scattering spectrum (red) due to inhomogeneity (green) of the nanodisk array.

$\sigma_D$  with particle size statistics (see Sec. S7 for details). Then,  $\sigma_\omega = \frac{d\omega}{dD} \sigma_D$ , where the slope  $\frac{d\omega}{dD}$  is obtained from the resonant frequencies  $\text{Re } \tilde{\omega}$  of the particles atop the gap of same thickness but with different diameters.

The real part of the resonant frequency  $\text{Re } \tilde{\omega}$  can be obtained straightforwardly—the center frequency of the Voigt profile, since the Lorentzian and Gaussian profiles are co-centered. The imaginary part  $\text{Im } \tilde{\omega}$  is obtained from Eqs. (S28) and (S29) via fitting to minimize root-mean-square error. Figures S10b and S10c shows two examples of the fitting process.

## B. Incorporation of inhomogeneous broadening in theoretical calculations for Si nanodisks

In Fig. 4d, in order to directly compare with measured spectra, the theoretical calculations (both non-classical and classical) of the scattering cross-sections of the Si disks also incorporates the broadening due to disk size inhomogeneity. Such incorporation can be understood as the inverse process of that described in Sec. S12.A. Figure S10d shows an example of the consequence of broadening due to nanodisk inhomogeneity, which contributes to an extra 6% broadening on the linewidth of the Si nanodisks.

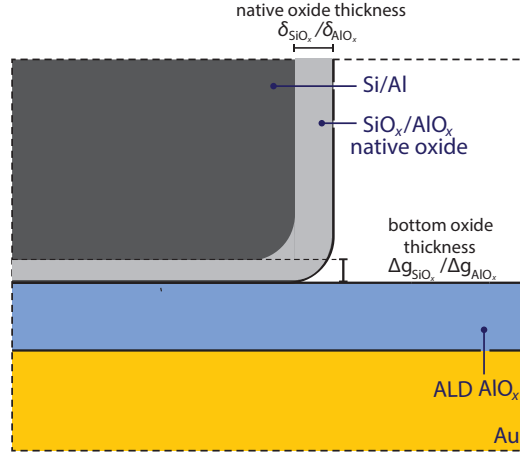

**Figure S11. Native oxide bottom layer of Al and Si nanodisks.**

### C. Oxide layers of Si and Al nanodisks

Unlike Au, both Al and Si oxidize in ambient conditions, adding extra uncertainty to the structural parameters of the resonators (see Fig. S11). For our Al and Si nanodisks, the top and side surfaces are fully exposed to air; therefore, the native oxide thickness  $\delta_\tau$  ( $\tau \in \{\text{SiO}_x, \text{AlO}_x\}$ ) should follow that in our ellipsometry measurement (see Supplementary section S9).

On the other hand, the bottom surface of the nanodisk does not expose to air (oxygen) directly; however, it may still form an oxide layer (thickness denoted by  $\Delta g_\tau$ ,  $\tau \in \{\text{SiO}_x, \text{AlO}_x\}$ ) by reacting with diffused oxygen since the ALD  $\text{AlO}_x$  layers are only few nanometer thick. Practically, we did not have a good in-situ method to directly measure the thickness of the bottom oxide.

For Si,  $\delta_{\text{SiO}_x} \approx 1.5$  nm as of measurement (see Supplementary section S9). We account for the uncertainty of the disk bottom oxide thickness by  $\Delta g_{\text{SiO}_x} \in (0, \delta_{\text{SiO}_x}]$ , since the bottom oxide should be no thicker than the native oxide (which is fully exposed to oxygen). Such structural uncertainty is taken into account by the uncertainty of the theoretical calculations of the resonant eigenfrequencies in both classical and nonclassical considerations (see Fig. 4c).

For Al, the measured native oxide  $\delta_{\text{AlO}_x} \approx 4$  nm (see Supplementary section S9). For such wide thickness, the applicability of the uncertainty analysis (as in the Si case) becomes limited. As an alternative, we adopt single-parameter fitting for the bottom native oxide layer with the model  $\Delta g_{\text{AlO}_x} = \delta_{\text{AlO}_x} e^{-\kappa g / \delta_{\text{AlO}_x}}$ , where  $g$  is the thickness of the ALD  $\text{AlO}_x$  spacer. In this model,  $\kappa$  is the only free parameter. We choose this model because of its reasonable asymptotics— $\lim_{g \rightarrow \infty} \Delta g_{\text{AlO}_x} = 0$  and  $\lim_{g \rightarrow 0} \Delta g_{\text{AlO}_x} = \delta_{\text{AlO}_x}$ . The first asymptotic means that sufficiently thick ALD  $\text{AlO}_x$  can already passivate the bottom surface of the Al disk, and the extra bottom oxide should vanish. The second asymptotic means that without the passivation from the ALD  $\text{AlO}_x$ , the bottom surface, like other surfaces of the disk, should develop oxide layer of similar thickness. We adopt  $\kappa = 0.6$  in the model to compare with our experimental results for Al (see Supplementary Sec. S15).

### S13. INDEX DEPENDENCE OF $d_{\perp}^{\text{Au-AlO}_x}$

The magnitude of the measured surface response functions depends on frequency and the materials that compose the interface [S12] (see also Sec. S16). In our measurements, due to the thickness-dependent refractive index ( $n_{\text{AlO}_x}$ ) of the  $\text{AlO}_x$  spacer (see Sec. S9 and Fig. 3d), the measured  $d_{\perp}^{\text{Au-AlO}_x}$ -parameter (Fig. 3b,c) inherits an effective  $n_{\text{AlO}_x}$ -dependence in addition to its frequency dependence.

In practice, we only sample a narrow slice of the entire  $(\tilde{\omega}, n_{\text{AlO}_x})$ -space, given the finite selection of  $(g, D)$ -combinations considered (and the associated resonance dispersion with  $g$  and  $D$ ). The resolu-

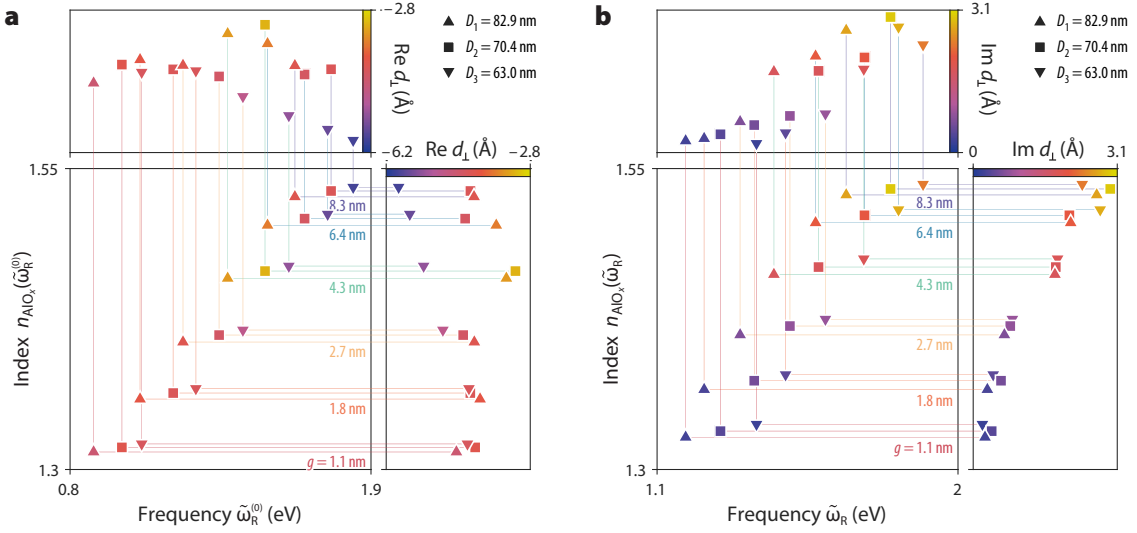

**Figure S12. Frequency and index dependence of measured  $d_{\perp}^{\text{Au-AIO}_x}$ .** Feibelman  $d$ -parameters generally depend on both frequency and interface composition. Since the cladding response ( $n_{\text{AIO}_x}$ ) varies with gap-size (Sec. S9), the measured  $d_{\perp}^{\text{Au-AIO}_x}$  inherits this dependence, leading to an approximate overall  $(\tilde{\omega}_R, n_{\text{AIO}_x})$ -dependence (here,  $\tilde{\omega}_R \equiv \text{Re } \tilde{\omega}$ ). Our measurements of **a.**  $\text{Re } d_{\perp}^{\text{Au-AIO}_x}$  and **b.**  $\text{Im } d_{\perp}^{\text{Au-AIO}_x}$  reveal the surface-response dispersion along the thin  $(\tilde{\omega}_R, n_{\text{AIO}_x})$ -band sampled by our 18  $(g, D)$ -combinations. For  $\text{Re } d_{\perp}^{\text{Au-AIO}_x}$  the perturbation centers are the classical eigenfrequencies, i.e.  $(\tilde{\omega}_R^{(0)}, n_{\text{AIO}_x}(\tilde{\omega}_R^{(0)}))$ ; for  $\text{Im } d_{\perp}^{\text{Au-AIO}_x}$  the perturbation centers are chosen as the measured eigenfrequencies, i.e.  $(\tilde{\omega}_R, n_{\text{AIO}_x}(\tilde{\omega}_R))$ , cf. the largeness of the nonclassical  $\tilde{\omega}_R^{(1)}$ -correction (see Sec. 2).

tion limitation of fabrication—joint constraints from electron beam lithography and lift-off processes—restricts us from decreasing the disk diameters. On the other hand, the long-wavelength cut-off ( $\approx 1500$  nm) of the spectrometer restricts us from increasing the disk diameters.

The dispersion of  $d_{\perp}^{\text{Au-AIO}_x}$  along this slice is shown in Fig. S12, illustrating the various “projection”-perspectives one may consider. As noted, the  $(\tilde{\omega}, n_{\text{AIO}_x})$ -space sampled by our measurements resembles a relatively thin band: the narrowness of this band precludes us from simultaneously disentangling both dependencies separately. Therefore, the linear frequency-fits in Figs. 3b,c ultimately reflect a composite dependence along the sampled  $(\tilde{\omega}, n_{\text{AIO}_x})$  space.

#### S14. ADDITIONAL MEASURED SI SCATTERING SPECTRA

In Fig. 4d, we show the measured spectra and optical response robustness for the thinnest gap 1.1 nm. Here in Fig. S13 we include additional measurement and comparisons with nonclassical and classical simulations to further demonstrate the robustness. Again, we observe minor nonclassical corrections.

#### S15. AL-AU RESULTS: PARTIAL CANCELLATION OF NONCLASSICAL CORRECTIONS BETWEEN SPILL-IN/OUT MATERIALS

Here in Fig. S14a–l, we demonstrate the cancellation of nonclassical corrections from different materials of spill-in or spill-out induced charge density (i.e. opposite signs of  $\text{Re } d_{\perp}$ ). The spill-in material is chosen as Au, whose surface response function is taken from our measurement (Fig. 3). The spill-out material is chosen as Al and its surface response function is obtained from TDDFT calculation of lossless homogeneous electron gas of Wigner-Seitz radius  $r_s = 2$  (Supplementary Section S16).

The scattering spectra of 18 Al nanodisk arrays were collected (Fig S14a,e,i), spanning three diameters and six gaps sizes. Following the same data analysis approach (see Sec. S12), we obtain the the measured complex resonant frequencies. As shown in Fig. 4b,f,k we theoretically predict that the Au substrate and

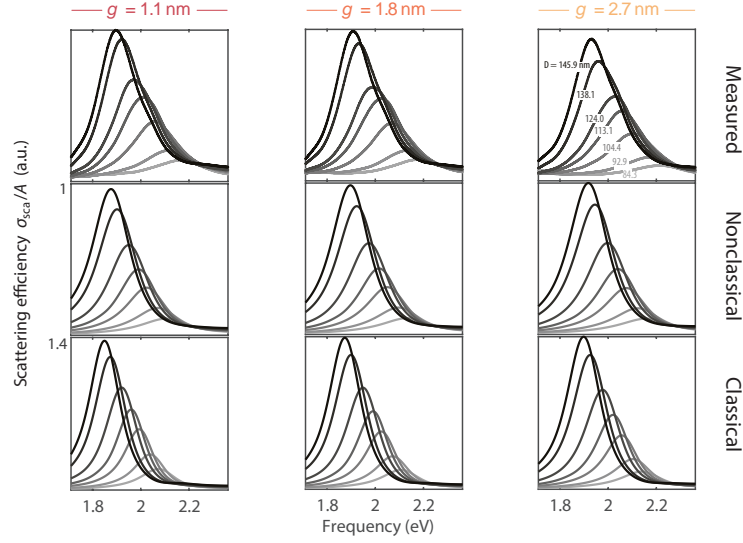

**Figure S13. Additional measurement showing robustness to nonclassical corrections from Si nanodisks with gap sizes of 1.1 nm, 1.8 nm, and 2.7 nm.**

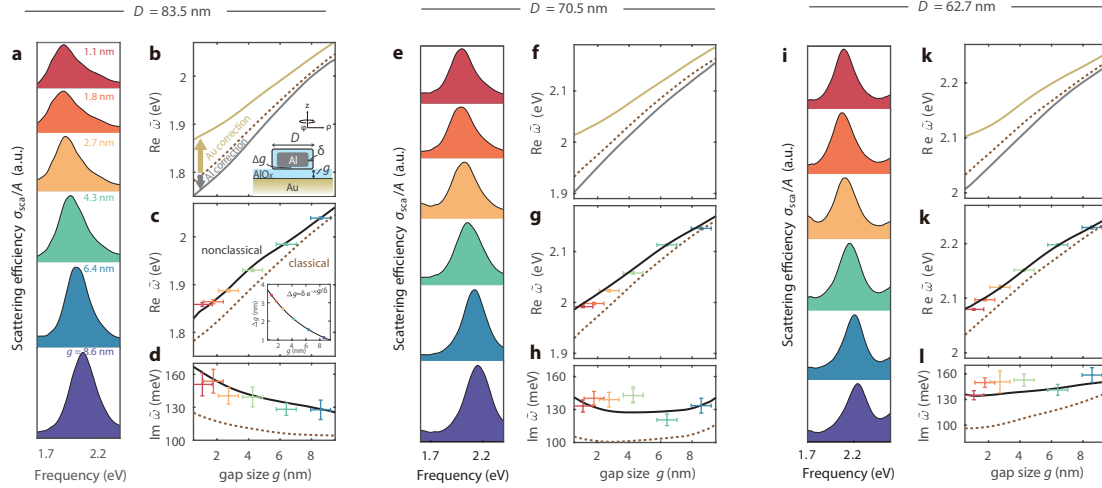

**Figure S14. Cancellation of nonclassical corrections in Au-film-coupled Al nanodisks** (structure and disk-bottom oxide modeling shown in **b–c** insets). Complex resonant frequencies obtained from per-volume scattering cross-sections (**a**, **e** and **i**) are in agreement with nonclassical calculations (solid black lines in **c–d**, **g–h**, and **k–l**), indicating the cancellation between the nonclassical corrections from the spill-in (Au) and spill-out (Al) materials (**b**, **f**, and **k**).

the Al nanodisk introduce blueshift and redshift nonclassical corrections respectively, and partially cancel with each other. The total nonclassical shift is still blueshift due to the more pronounced correction from Au, and agrees with our measurement (Fig. 4c,g,k). Despite the cancellation in  $\text{Re } \tilde{\omega}$ , passivity requires that the spectral broadening is still cumulative for  $\text{Im } \tilde{\omega}$  (Fig. 4d,h,l). In these theoretical calculations, we include an exponential bottom-disk oxide model with a single free parameter  $\kappa$  for both classical and nonclassical considerations (see Fig. S14b,c insets and Sec. S12.C). The same model is applied to the results of three discrete Al disk diameters, which yields similar agreement between experiment and theory. We also note that the prediction of nonclassical correction cancellation is unaffected by the choice of bottom-oxide layer model.

## S16. TDDFT: IMPACT OF CLADDING SCREENING ON $d$ -PARAMETERS

The measured  $d_{\perp}$  of the Au–AlO<sub>x</sub> interface shows a comparatively high magnitude, specifically its real part ranges from  $-0.5$  nm to  $-0.4$  nm over frequencies from  $0.9$  eV to  $1.8$  eV (Fig. 3b). In this section, using time-dependent density functional theory (TDDFT), we identify and explain the physical mechanism responsible for this large magnitude: screening of the cladding material (AlO<sub>x</sub>) increases the magnitude of  $d_{\perp}$ . In noble metals, the increase is approximately linear with cladding permittivity.

The TDDFT calculations to be discussed incorporate three central approximations common to virtually all published studies of  $d$ -parameters (e.g. [S4; S7; S12])

1. The jellium approximation of the positive ionic background.
2. The semiclassical screening approximation (SCSA) of valence electrons.
3. The adiabatic local density approximation of the exchange-correlation energy.

Despite its relative coarseness, especially points 1 and 2, such a treatment in fact exemplifies the state-of-the-art for computation of  $d$ -parameters. Specifically, with the second approximation, the SCSA, we characterize the screening of valence electrons in terms of a polarizable medium with a local permittivity. These approximations greatly benefit computational simplicity at the cost of two primary drawbacks: (i) neglecting crystalline and band structure effects, and (ii) coarsely approximating the conduction–valence polarization interaction near the metal–dielectric interface. The second drawback is sufficiently non-negligible that it renders *quantitative* predictions for  $d_{\perp,\parallel}$  unattainable, except for simple metals where the conduction–valence polarization interaction is negligible or non-existent [S26]. Nevertheless, these drawbacks do not hinder the objective of this section: assessing the qualitative impact of screening from the cladding medium on the relative magnitude of  $d$ -parameters.

### A. Qualitative analysis

A qualitative understanding of the impact of the cladding screening on  $d_{\perp}$  can be drawn from the following arguments. Let us consider a metal–dielectric system: the uniform positive ionic background—a built-in assumption in the jellium approximation—of the metal occupies the half space  $x < 0$ , while the other half space  $x > 0$  is occupied by a dielectric cladding medium. A uniform electric field oriented perpendicular to the metal–dielectric interface drives the system. The SCSA permits us to partition the induced electronic polarization into the contributions from the metal and the cladding dielectric medium, which are denoted by  $\mathbf{P}_m$  and  $\mathbf{P}_d$ , respectively. Accordingly, the induced charge density  $\rho$  can be expressed as a summation of metallic and dielectric contributions,  $\rho = \rho_m + \rho_d$ , via the relations  $\rho_{m,d} = -\epsilon_0^{-1} \partial_x \mathbf{P}_{m,d}$ . In turn, the centroid of the total induced charge  $d_{\perp} \equiv \int x \rho(x) dx / \int \rho(x) dx$  can be expressed as a weighted average of the centroids of  $\rho_m$  and  $\rho_d$ —that is, of  $d_{\perp,m} \equiv \int x \rho_m(x) dx / \int \rho_m(x) dx$  and  $d_{\perp,d} \equiv \int x \rho_d(x) dx / \int \rho_d(x) dx$ —such that

$$d_{\perp} = f_m d_{\perp,m} + f_d d_{\perp,d}, \quad (\text{S30})$$

with the weighting factors<sup>‡‡</sup>

$$f_m \equiv \frac{\int_{-\infty}^{\infty} \rho_m(x) dx}{\int_{-\infty}^{\infty} \rho(x) dx} = \frac{\epsilon_d - \epsilon_d/\epsilon_m}{1 - \epsilon_d/\epsilon_m} + O(k), \quad (\text{S31a})$$

$$f_d \equiv \frac{\int_{-\infty}^{\infty} \rho_d(x) dx}{\int_{-\infty}^{\infty} \rho(x) dx} = 1 - f_m = \frac{1 - \epsilon_d}{1 - \epsilon_d/\epsilon_m} + O(k). \quad (\text{S31b})$$

In our Au nanoparticle experiment (Fig. 3 of the main text) we find  $|\epsilon_d/\epsilon_m|$  ranging from about 0.02

<sup>‡‡</sup> At the last equality signs, we exploit that the aggregate classically induced charge equals the aggregate quantum-mechanically induced charge in the  $k \rightarrow 0$  limit. Thus,  $f_m$  and  $f_d$  are classical quantities within the first-order scope of Feibelman  $d$ -parameters. Classically,  $\rho_m(x) = 2\epsilon_0 k [\epsilon_d(1 - \epsilon_m)/(\epsilon_m + \epsilon_d)] \delta(x)$  and  $\rho_d(x) = 2\epsilon_0 k [\epsilon_m(\epsilon_d - 1)/(\epsilon_m + \epsilon_d)] \delta(x)$  for  $\phi^{\text{ext}}(x) = e^{iky+kx}$  [S4].

at  $\hbar\omega = 0.9$  eV to about 0.15 at  $\hbar\omega = 1.8$  eV. The negligible value of  $|\varepsilon_d/\varepsilon_m|$  justifies the simplifying approximations  $f_m \approx \varepsilon_d$  and  $f_d \approx 1 - \varepsilon_d$ , showing that  $f_m > 0$  while  $f_d < 0$ .

We now examine the relation between  $d_\perp$  and  $d_\perp^{\text{vacuum}}$ , with the latter being the centroid of induced charge at the metal–vacuum interface. To emphasize the relative impact of cladding screening clearly, we introduce the dimensionless quantity  $\tilde{d}_\perp$ :

$$\tilde{d}_\perp \equiv \frac{d_\perp}{d_\perp^{\text{vacuum}}} \approx \frac{d_\perp}{d_{\perp,m}} \approx f_m + f_d \frac{d_{\perp,d}}{d_{\perp,m}}, \quad (\text{S32})$$

where the approximation  $d_\perp^{\text{vacuum}} \approx d_{\perp,m}$  has been employed, which is exact when the cladding screening vanishes, i.e. when  $\varepsilon_d = 1$ . In the SCSA, for an independent dielectric medium, i.e. a dielectric–vacuum semi-infinite system  $d_{\perp,d} = 0$ , because  $\rho_d$  is the Dirac delta function localized at  $x = 0$ . Attaching a metal to a dielectric, the tail of  $\rho_m$ , contributed from conduction electrons of the metal that spread into the dielectric medium, shall induce a smooth electronic distribution of  $\rho_d$ , thereby rendering  $d_{\perp,d}$  non-zero. For “spill-in” materials, such as Au with  $\text{Re } d_{\perp,m} < 0$ ,<sup>§§</sup> it is proper to assume  $d_{\perp,d}$  being negligible, since  $\rho_m$  is mostly located inside the metal and, accordingly, the induced  $\rho_d$  due to the overlap between  $\rho_m$  and the dielectric medium is expected to be negligible. Thus, for Au, we deduce that Eq. (S32) can be further approximated to

$$\tilde{d}_\perp \approx \varepsilon_d, \quad (\text{S33})$$

where we have used the approximation  $f_m \approx \varepsilon_d$ . Equation (S33) shows that the cladding screening increases  $d_\perp$  by a factor of  $\varepsilon_d$  with respect to  $d_\perp^{\text{vacuum}}$ . Concerning our experiment, in which  $\varepsilon_d$  ranges from  $\approx 1.7$  to  $\approx 2.3$ , we thus deduce that the magnitude of  $d_\perp^{\text{Au–vacuum}}$ , the centroid of the induced charge density of the Au–vacuum interface, is about two times smaller than  $d_\perp^{\text{Au–AlO}_x}$ . Specifically,  $\text{Re } d_\perp^{\text{Au–vacuum}} \approx -0.2$  nm.

Finally, we note that, for “spill-out” materials, such as Al, of which  $\rho_m$  is mostly located outside the metal with  $\text{Re } d_{\perp,m} > 0$ , Eq. (S33) becomes invalid, since the last term  $f_d d_{\perp,d}/d_{\perp,m}$  in Eq. (S32) cannot be dropped. Moreover, we can deduce that  $f_d \text{Re } d_{\perp,d}/\text{Re } d_{\perp,m} < 0$ ,<sup>¶¶</sup> and this term (neglecting the imaginary parts of  $d_{\perp,d}$  and  $d_{\perp,m}$ ) neutralizes the positive term  $f_m$ , and, accordingly, reduce the impact of the cladding screening, as evidenced with numerical results later.

## B. Numerical results

### Implementation

Numerical techniques for the application of TDDFT to the calculation of  $d$ -parameters has been expounded in several papers [S4; S7; S12]. For completeness, we here present a brief summary of key points in our implementation.

We consider a metallic slab with length  $L$  surrounded by a dielectric medium. The uniform positive ionic background of the metal is located in the region  $-L/2 < x < L/2$  and has a density of  $n_{\text{ion}}$  equal to the density of the conduction electrons of the metal. Notably,  $L$  should be set to be large enough such that the computed  $d_\perp$  converges to its limiting value as  $L \rightarrow \infty$ ; in our numerical examples, shown below, we choose  $L = 10$  nm.

According to the SCSA, the screening of the valence electrons of the metal and the background dielectric

<sup>§§</sup> We infer that  $\text{Re } d_\perp^m < 0$  for Au by the following arguments: 1.  $\text{Re } d_\perp < 0$  is observed experimentally; 2.  $\rho_d$  is due to the polarization of the valence electrons in the half space  $x > 0$ , thus  $\text{Re } d_{\perp,d} > 0$ ; and 3. given this, and the fact that  $f_d < 0$ , we find that  $\text{Re } d_{\perp,m} < 0$  cf. Eq. (S30).

<sup>¶¶</sup>  $f_d \text{Re } d_{\perp,d}/\text{Re } d_{\perp,m} < 0$  is deduced by the following arguments: 1.  $f_d < 0$ , seen from its expression; 2.  $\text{Re } d_{\perp,m} < 0$  for simple metals below the multipolar flat-surface plasmon frequency, roughly  $0.8\omega_p$ , which, for Al, is about 13.34 eV; 3.  $\text{Re } d_{\perp,d} > 0$  since  $\rho_d$  localizes in the dielectric medium; and 4. combining the above considerations, we deduce  $f_d \text{Re } d_{\perp,d}/\text{Re } d_{\perp,m} < 0$

medium is included through a step-wise permittivity profile:

$$\varepsilon_s(x, \omega) = \begin{cases} \varepsilon_m^b(\omega) & |x| < L/2, \\ \varepsilon_d(\omega) & |x| > L/2. \end{cases} \quad (\text{S34})$$

For simple metals, such as Na and Al, the screening from the valence electrons can be neglected across optical frequencies, rendering  $\varepsilon_m^b = 1$ . For Au, the contribution from the 5d valence-electrons is significant; we infer  $\varepsilon_m^b$  approximately from our ellipsometrically measured Au permittivity (see Fig. S15).\*\*\*

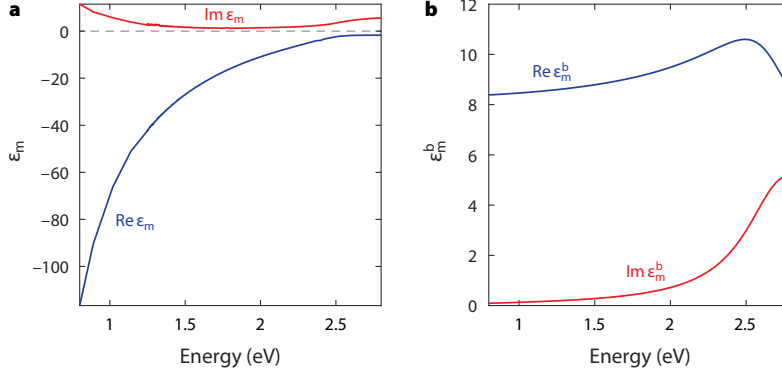

**Figure S15. Valence-electron contribution to dielectric response of Au.** **a.** Au permittivity ( $\varepsilon_m$ ) as measured ellipsometrically (Sec. S9). **b.** Inferred bound-screening contribution ( $\varepsilon_m^b$ ) of Au due to valence electrons.\*\*\*

To study response dynamics, we perturb the system in the linear regime with an external electric potential  $\phi_{\text{ext}}(x, \omega, k_{\parallel})e^{i\mathbf{k}_{\parallel} \cdot \mathbf{r}_{\parallel} - i\omega t}$ , where  $\mathbf{r}_{\parallel} \equiv y\hat{y} + z\hat{z}$  incorporates the in-plane dependence. We design  $\phi_{\text{ext}}$  such that

$$\phi_{\text{ext}}(x, \omega, k_{\parallel}) = \begin{cases} e^{k_{\parallel}x} + r_s(\omega, k_{\parallel})e^{-k_{\parallel}x} & x > L/2, \\ a_s(\omega, k_{\parallel})e^{k_{\parallel}x} + b_s(\omega, k_{\parallel})e^{-k_{\parallel}x} & |x| < L/2, \\ t_s(\omega, k_{\parallel})e^{k_{\parallel}x} & x < -L/2, \end{cases} \quad (\text{S35})$$

representing the potential generated by  $e^{k_{\parallel}x}$  impinging from the region  $x > L/2$  upon the dielectric environment  $\varepsilon_s(x, \omega)$ , where  $k_{\parallel} = |\mathbf{k}_{\parallel}|$ . The coefficients  $r_s$ ,  $a_s$ ,  $b_s$  and  $t_s$  are straightforwardly determined by matching the boundary conditions (continuity of  $\phi_{\text{ext}}$  and  $-\varepsilon_s \partial_x \phi_{\text{ext}}$  across  $x = \pm L/2$ ).

We solve the induced density of the conduction electrons,  $\delta n_{-}(x, \omega, k_{\parallel})e^{i\mathbf{k}_{\parallel} \cdot \mathbf{r}_{\parallel} - i\omega t}$ , by

$$\delta n_{-}(x, \omega, k_{\parallel}) = -e \int \chi(x, x'; \omega, k_{\parallel}) \phi_{\text{ext}}(x, \omega, k_{\parallel}) dx'. \quad (\text{S36})$$

\*\*\* The  $\varepsilon_m^b(\omega)$  contribution is inferred by following procedure:

1. A Lorentz-Drude form is assumed for the total dielectric response, i.e.  $\varepsilon_m(\omega) \equiv \varepsilon_m^b(\omega) - \omega_{p,D}^2/(\omega^2 + i\omega\gamma_D)$ ; here, the Drude term  $\{\omega_{p,D}, \gamma_D\}$  accounts response from conduction electrons while  $\varepsilon_m^b(\omega) \equiv \varepsilon_{\infty} - \sum_{n=1}^2 \omega_{p,n}^2/(\omega^2 - \omega_{0,n}^2 + i\omega\gamma_n)$  accounts for bound-screening due to valence electrons (through two Lorentz oscillator terms  $\{\omega_{p,n}, \omega_{0,n}, \gamma_n\}$  and a constant bias  $\varepsilon_{\infty}$ ).
2. The conduction-electron density ( $n_{\text{ion}} = 5.9 \times 10^{28} \text{ m}^{-3}$ ) determines the (unscreened) Drude plasma frequency  $\omega_{p,D} \equiv (e^2 n_{\text{ion}} / \varepsilon_0 m_e)^{1/2} \approx 9.0195 \text{ eV}$ .
3. The Drude damping rate  $\hbar\gamma_D \approx 69.4 \text{ meV}$  is extracted by fitting the measured  $\text{Im } \varepsilon_m(\omega)$  to the  $\omega \gg \gamma_D$  Drude-approximation  $\text{Im } \varepsilon_m(\omega) \approx \omega_{p,D}^2 \gamma_D / \omega^3$  across  $\hbar\omega \in [0.6 \text{ eV}, 1.5 \text{ eV}]$ . This approximation is excellent over the considered energy range since  $\text{Im } \varepsilon_m^b \approx 0$  below the onset of d-electron interband transitions (at  $\approx 1.6 \text{ eV}$ , above which  $\text{Im } \varepsilon_m$  increases noticeably).
4. The Lorentz and constant-bias parameters are extracted by fitting to  $\varepsilon_m^b(\omega) = \varepsilon_m(\omega) + \omega_{p,D}^2/(\omega^2 + i\omega\gamma_D)$  (uniquely determined by our measurements and the aforementioned Drude parameters): we obtain  $\varepsilon_{\infty} \approx 6.703$ ,  $\hbar\omega_{p,1} \approx 5.765 \text{ eV}$ ,  $\hbar\omega_{p,2} \approx 7.795 \text{ eV}$ ,  $\hbar\omega_{0,1} \approx 2.7362 \text{ eV}$ ,  $\hbar\omega_{0,2} \approx 3.1387 \text{ eV}$ ,  $\hbar\gamma_1 \approx 0.5772 \text{ eV}$ , and  $\hbar\gamma_2 \approx 0.5118 \text{ eV}$ .

The interacting nonlocal response function  $\chi$  is given by

$$\chi(x, x'; \omega, k_{\parallel}) = \chi^0(x, x'; \omega, k_{\parallel}) + \iint \chi^0(x, x_1; \omega, k_{\parallel}) \left[ -e^2 g(x_1, x_2; \omega, k_{\parallel}) + f_{xc}[n_-](x_1, x_2; \omega) \right] \chi(x_2, x'; \omega, k_{\parallel}) dx_1 dx_2, \quad (\text{S37})$$

with  $f_{xc}[n_-](x_1, x_2; t - t') \equiv \frac{\delta V_{xc}[n_-](x_1, t)}{\delta n_-(x_2, t')}$ ; within ALDA, its frequency-representation simplifies to  $f_{xc}[n_-](x_1, x_2; \omega) = \frac{\delta V_{xc}[n_-(x_1, \omega)]}{\delta n_-(x_2, \omega)} \delta(x_1 - x_2)$ , where  $V_{xc}$  is chosen as the (LDA) Gunnarsson–Lundqvist xc-functional [S27].  $g(x, x'; \omega, k_{\parallel})$  is the Green's function of the 1D Poisson equation:

$$\frac{d}{dx} \left[ \epsilon_s(x, \omega) \frac{d}{dx} - k_{\parallel}^2 \epsilon_s(x, \omega) \right] g(x, x'; \omega, k_{\parallel}) = \delta(x - x'). \quad (\text{S38})$$

Lastly, the noninteracting response function  $\chi^0$  can be constructed directly from the ground-state orbitals of the conduction electrons [S26; S28].

One existing approach to compute  $d_{\perp}$  exploits the dynamic-force sum rule, as proposed by Liebsch, to bypass the numerical difficulty of the direct evaluation of  $d_{\perp}$  due to Friedel oscillations of the induced charge that decay slowly inside the metal. Though Liebsch's approach in principle is suitable for our current problem, it is not immediately applicable to beyond-jellium calculations of the  $d$ -parameters that explicitly incorporate the lower-lying valence orbitals. An extension to the state-of-the-art  $d$ -parameter computation technique remains yet to be explored.

Motivated by breaking down the limitations of Liebsch's approach—a requirement for beyond-jellium  $d$ -parameter calculations—we here propose a distinct approach, inspired by ellipsometry, in which  $d$ -parameters are determined by comparing the reflection and transmission coefficients of the metal slab obtained from the TDDFT calculations to our proposed mesoscopic model. Specifically, after obtaining  $\delta n_-$ , we compute the total electric potential

$$\phi_{\text{tot}}(x, \omega, k_{\parallel}) = \phi_{\text{ext}}(x, \omega, k_{\parallel}) + \phi_{\text{ind}}(x, \omega, k_{\parallel}), \quad (\text{S39})$$

where  $\phi_{\text{ind}}$ , the induced potential by  $\delta n_-$  in the dielectric environment  $\epsilon_s$ , is given by

$$\phi_{\text{ind}}(x, \omega, k_{\parallel}) = \int \delta n_-(x', \omega, k_{\parallel}) g(x, x'; \omega, k_{\parallel}) dx'. \quad (\text{S40})$$

Then, we extract the reflection and transmission coefficients of the metal slab, denoted by  $r_{\text{tot}}$  and  $t_{\text{tot}}$ , respectively, from  $\phi_{\text{tot}}$ , which, for points far away from the metal slab  $x \gg |L|/2$ , takes the asymptotic form

$$\phi_{\text{tot}}(x, \omega, k_{\parallel}) = \begin{cases} e^{k_{\parallel}x} + r_{\text{tot}}(\omega, k_{\parallel}) e^{-k_{\parallel}x} & x \gg L/2, \\ t_{\text{tot}}(\omega, k_{\parallel}) e^{k_{\parallel}x} & x \ll -L/2. \end{cases} \quad (\text{S41})$$

On the other hand, we employ the mesoscopic model—in which the  $d$ -parameters modify the boundary conditions at the metal-interface according to Eqs. (1) in the main text—to find the expressions of the reflection and transmission coefficients of the metal slab in terms of the  $d$ -parameters. By requiring that the reflection and transmission coefficients from the mesoscopic model equal the  $r_{\text{tot}}$  and  $t_{\text{tot}}$  obtained from the TDDFT calculations, we determine both  $d_{\perp}$  and  $d_{\parallel}$ .

Based on the approach described above, next we use two examples, Au and Al (two metals studied in this work), to show the impact of the cladding screening. Again, we note that the absolute numerical values of  $d_{\perp}$  of Au obtained from our TDDFT jellium calculations do not possess quantitative accuracy, due to the reasons explained at the beginning of this section. Therefore, only the normalized dimensionless quantity  $\tilde{d}_{\perp}$  is shown in Figs. S16.

Au (noble metal): infinite-square-well model

We use  $\epsilon_m^b$  presenting in Fig. S15. Since the DFT jellium calculations of Au lacks accuracy due to non-negligible screening from lower-lying orbitals [S4; S6; S29], the work function of the Au-vacuum interface can be underestimated by several electron-volts. Consequently, the successive TDDFT calculations cannot produce meaningful  $d_{\perp}$  values, even on the qualitative level.

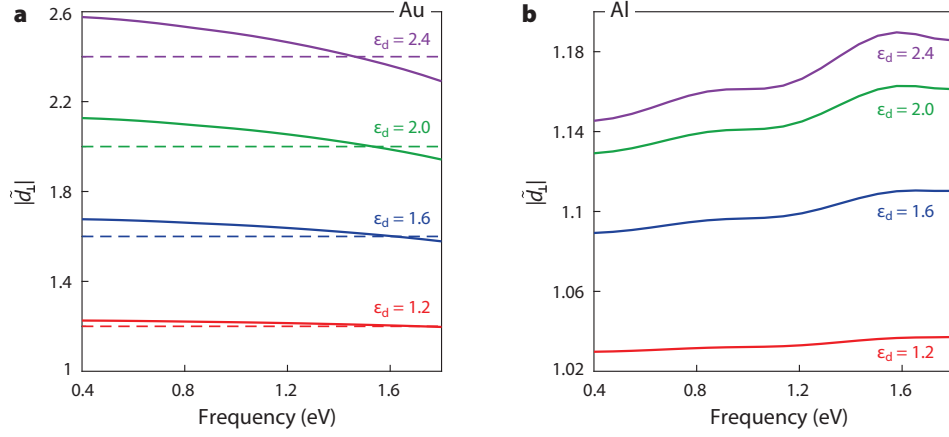

**Figure S16. Screening effect on  $d_{\perp}$ -parameter of Au and Al.** **a.** For Au, the enhancement of  $d_{\perp}$  (solid lines), i.e.,  $|\tilde{d}_{\perp}|$  agrees well with  $\epsilon_d$  (dashed lines), supporting the approximation of Eq. (S33). **b.** The impact of the cladding screening for Al is considerably weaker than Au, and is out of the valid regime of Eq. (S33).

Instead, we employ a toy model featuring the infinite square well approximation to treat the ground-state properties of Au. Such an infinite-square-well model ensures that  $\text{Re } d_{\perp}$  is always negative, since the conduction electrons are wholly confined to the metal region  $|x| < L/2$ . This treatment allows us to study the impact of the cladding screening on  $d_{\perp}$  for  $\text{Re } d_{\perp} < 0$ , corresponding to realistic Au as observed in our and previous experiments.

Specifically, the ground-state conduction electrons of Au are assumed confined by an infinite-well potential along  $x$ , namely by

$$V_{\text{eff}}(x) = \begin{cases} \infty & |x| > L/2, \\ 0 & |x| < L/2. \end{cases} \quad (\text{S42})$$

The ground-state orbitals are obtained by solving the Schrödinger equation under the potential  $V_{\text{eff}}$ , which are then used to construct the noninteracting response function  $\chi^0$ .

We vary the cladding permittivity  $\epsilon_d$ , sampling four different values  $\epsilon_d = 1.2, 1.6, 2, 2.4$ . Since we find that  $\tilde{d}_{\perp}$  is almost real-valued and  $\text{Re } \tilde{d}_{\perp}$  is positive for all values of  $\epsilon_d$  considered, we plot in Fig. S16a  $|\tilde{d}_{\perp}|$  (solid curves), which agrees well with a  $\epsilon_d$ -scaling (dashed curves). These results thus support our claim at the beginning of this section that the screening of the cladding medium increases the magnitude of  $d_{\perp}$  by a factor proportional to  $\epsilon_d$ .

Al (simple metal)

We set  $\epsilon_m^b = 1$ . The ground-state orbitals of the conduction electrons, used to construct the noninteracting response function  $\chi^0$ , are obtained from the self-consistent jellium DFT calculations. For Al, the jellium DFT results are quite accurate, e.g. the predicted the work function of Al-vacuum is 3.76 eV, close to the experimental value 4.06–4.26 eV. Fig. S16b plots  $|\tilde{d}_{\perp}|$  (solid curves) of Al, which, unlike those of Au, disagree with the prediction of Eq. (S33). We reiterate the explanation at the end of Sec. S16.A below. The prerequisite for Eq. (S33)—the induced charge of the metal should be primarily located in the metallic region, i.e.  $\text{Re } d_{\perp,d} < 0$ —no longer holds for simple “spill-out” metals like Al.

## References

- \* [yyi@mit.edu](mailto:yyi@mit.edu); [dizhu@mit.edu](mailto:dizhu@mit.edu); These authors contributed equally to this work.
- [S1] P.J. Feibelman, *Prog. Surf. Sci.* **12**, 287 (1982).
  - [S2] A. Liebsch, *Electronic Excitations at Metal Surfaces*, Physics of Solids and Liquids (Springer, 1997).
  - [S3] P. Apell, *Physica Scripta* **24**, 795 (1981).
  - [S4] T. Christensen, W. Yan, A.-P. Jauho, M. Soljačić, and N.A. Mortensen, *Phys. Rev. Lett.* **118**, 157402 (2017).
  - [S5] B.N.J. Persson and P. Apell, *Phys. Rev. B* **27**, 6058 (1983).
  - [S6] A. Liebsch, *Phys. Rev. B* **48**, 11317 (1993).
  - [S7] A. Liebsch and W.L. Schaich, *Phys. Rev. B* **52**, 14219 (1995).
  - [S8] P. Apell, R. Monreal, and F. Flores, *Solid State Commun.* **52**, 971 (1984).
  - [S9] L. Novotny and B. Hecht, *Principles of Nano-Optics* (Cambridge University Press, 2012).
  - [S10] J.D. Jackson, *Classical Electrodynamics*, 3rd ed. (John Wiley & Sons, 1999).
  - [S11] W. Yan, M. Wubs, and N. A. Mortensen, *Phys. Rev. Lett.* **115**, 137403 (2015).
  - [S12] D. Jin, Q. Hu, D. Neuhauser, F. von Cube, Y. Yang, R. Sachan, T.S. Luk, D.C. Bell, and N.X. Fang, *Phys. Rev. Lett.* **115**, 193901 (2015).
  - [S13] A. Ishimaru, *Electromagnetic wave propagation, radiation, and scattering: from fundamentals to applications*, 2nd ed. (John Wiley & Sons, 2017) pp. 357–399.
  - [S14] Y. Yang, O.D. Miller, T. Christensen, J.D. Joannopoulos, and M. Soljačić, *Nano Lett.* **17**, 3238 (2017).
  - [S15] P. Lalanne, W. Yan, K. Vynck, C. Sauvan, and J.-P. Hugonin, *Laser Photonics Rev.* **12**, 1700113 (2018).
  - [S16] J. Yang, H. Giessen, and P. Lalanne, *Nano Lett.* **15**, 3439 (2015).
  - [S17] S. Berciaud, L. Cognet, P. Tamarat, and B. Lounis, *Nano Lett.* **5**, 515 (2005).
  - [S18] C. Ciraci, X. Chen, J.J. Mock, F. McGuire, X. Liu, S.-H. Oh, and D.R. Smith, *Appl. Phys. Lett.* **104**, 023109 (2014).
  - [S19] H. Fujiwara, J. Koh, P.I. Rovira, and R.W. Collins, *Phys. Rev. B* **61**, 10832 (2000).
  - [S20] P. B. Johnson and R. W. Christy, *Phys. Rev. B* **6**, 4370 (1972).
  - [S21] T. Campbell, R. K. Kalia, A. Nakano, P. Vashishta, S. Ogata, and S. Rodgers, *Phys. Rev. Lett.* **82**, 4866 (1999).
  - [S22] S.M. George, *Chem. Rev.* **110**, 111 (2009).
  - [S23] M.D. Groner, J.W. Elam, F.H. Fabreguette, and S.M. George, *Thin Solid Films* **413**, 186 (2002).
  - [S24] A. Banerjee, R.M. Heath, D. Morozov, D. Hemakumara, U. Nasti, I. Thayne, and R.H. Hadfield, *Opt. Mater. Express* **8**, 2072 (2018).
  - [S25] B. Armstrong, *J. Quant. Spectrosc. Radiat. Transfer* **7**, 61 (1967).
  - [S26] A. Liebsch, *Phys. Rev. B* **36**, 7378 (1987).
  - [S27] O. Gunnarsson and B.I. Lundqvist, *Phys. Rev. B* **13**, 4274 (1976).
  - [S28] G. Giuliani and G. Vignale, *Quantum theory of the electron liquid* (Cambridge University Press, 2005).
  - [S29] P.J. Feibelman, *Phys. Rev. Lett.* **72**, 788 (1994).
